# Supplementary material for: ShadowHack: Hacking Shadows via Luminance-Color Divide and Conquer
Source: arXiv:2412.02545 source file (2025-03-28)
Supplement: Supplementary file 1 [file X_suppl.tex]

\clearpage
\setcounter{section}{1}

\section*{More Visual Results}
% \balance
% \section*{A. Architectures of Extension Experiments}

% \subsection*{A.1 Ablation Study of Decoupling Framework}
% During the ablation study on our decoupling framework, we explore the end-to-end network and the Retinex-based framework.
% For the end-to-end network, we adopt the same baseline as our models. With an input concatenated by RGB images and its shadow masks, the network outputs shadow-free images directly. 

% For the Retinex-based experiment, we first decompose the image to its illumination map and reflectance map. The decomposing model consists of a U-Net~\cite{RonnebergerFB15} and is trained with the loss function of L1 loss and WTV loss~\cite{GuoH23}. We obtain illumination maps from the U-Net and their reflectance maps via division. Subsequently, we relight the illumination and remove the color bias in reflectance with the same architecture as LRNet. 

% \subsection*{A.2 Mask Refine Network}
% The mask refine network simply adopts a U-Net~\cite{RonnebergerFB15}. We take $I_t$ and shadow mask as inputs and the refined mask will be generated. Considering the complexity of shadow characteristics, we inject ConvNext-v2 atto model~\cite{0003MWFDX22} as our CRNet does. The extracted features of RGB inputs are fed into the U-Net decoder for a more precise mask. 

% \section*{C. More Visual Results}

\begin{figure*}[h!]
    \centering
    
    \includegraphics[width=.20\linewidth]{fig/4/istd/115/115-8-input.jpg}
    \includegraphics[width=.20\linewidth]{fig/4/istd/115/115-8-BMNet.jpg}
    \includegraphics[width=.20\linewidth]{fig/4/istd/115/115-8-SG.jpg}
    \includegraphics[width=.20\linewidth]{fig/4/istd/115/115-8-shadowformer.jpg}

    \begin{subfigure}{0.20\linewidth}
        \centering
        \subcaption{Input}
    \end{subfigure}
    \begin{subfigure}{0.20\linewidth}
        \centering
        \subcaption{BMNet~\cite{ZhuHFZSZ22}}
    \end{subfigure}
    \begin{subfigure}{0.20\linewidth}
        \centering
        \subcaption{SG~\cite{WanYWWLW22}}
    \end{subfigure}
    \begin{subfigure}{0.20\linewidth}
        \centering
        \subcaption{SF~\cite{GuoHLCW23}}
    \end{subfigure}
    
    \includegraphics[width=.20\linewidth]{fig/4/istd/115/115-8-homo.jpg}
    \includegraphics[width=.20\linewidth]{fig/4/istd/115/115-8-rasm.jpg}
    \includegraphics[width=.20\linewidth]{fig/4/istd/115/115-8-ours.jpg}
    \includegraphics[width=.20\linewidth]{fig/4/istd/115/115-8-gt.jpg}
    
    \begin{subfigure}{0.20\linewidth}
        \centering
        \subcaption{HF~\cite{0002FZL00Z24}}
    \end{subfigure}
    \begin{subfigure}{0.20\linewidth}
        \centering
        \subcaption{RASM~\cite{liu2024regional}}
    \end{subfigure}
    \begin{subfigure}{0.20\linewidth}
        \centering
        \subcaption{Ours}
    \end{subfigure}
    \begin{subfigure}{0.20\linewidth}
        \centering
        \subcaption{GT}
    \end{subfigure}

    \includegraphics[width=.20\linewidth]{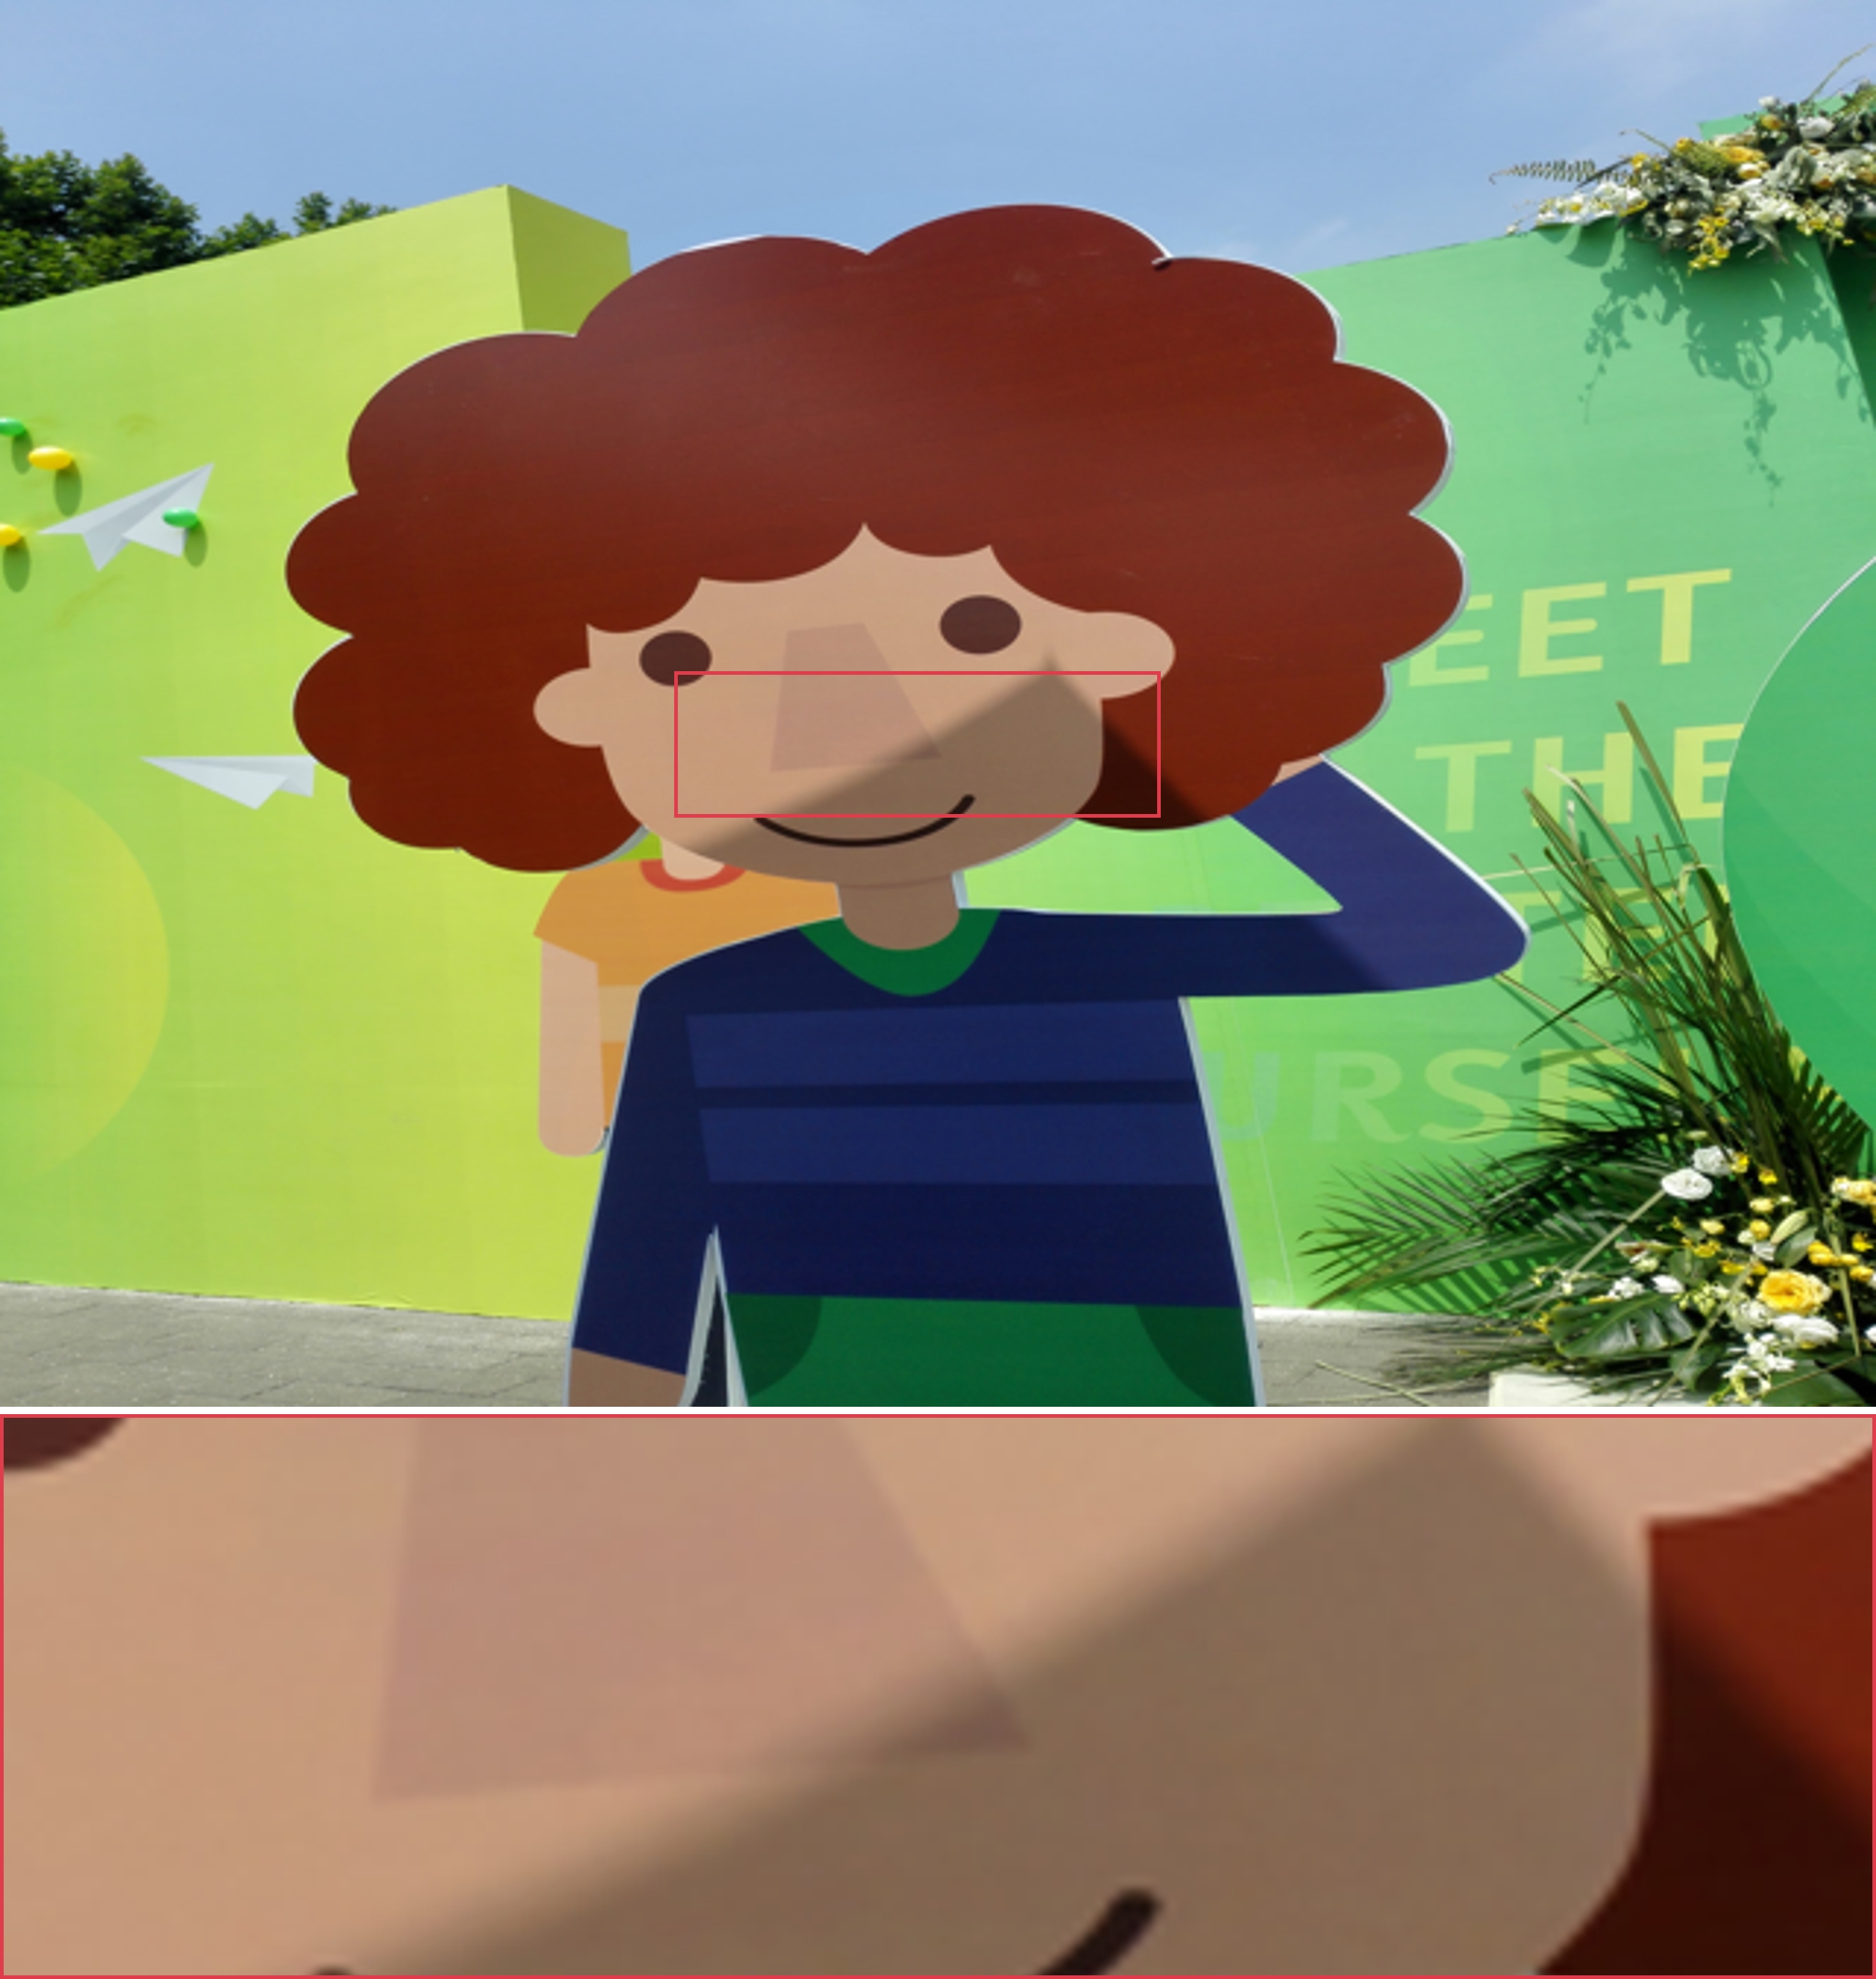}
    \includegraphics[width=.20\linewidth]{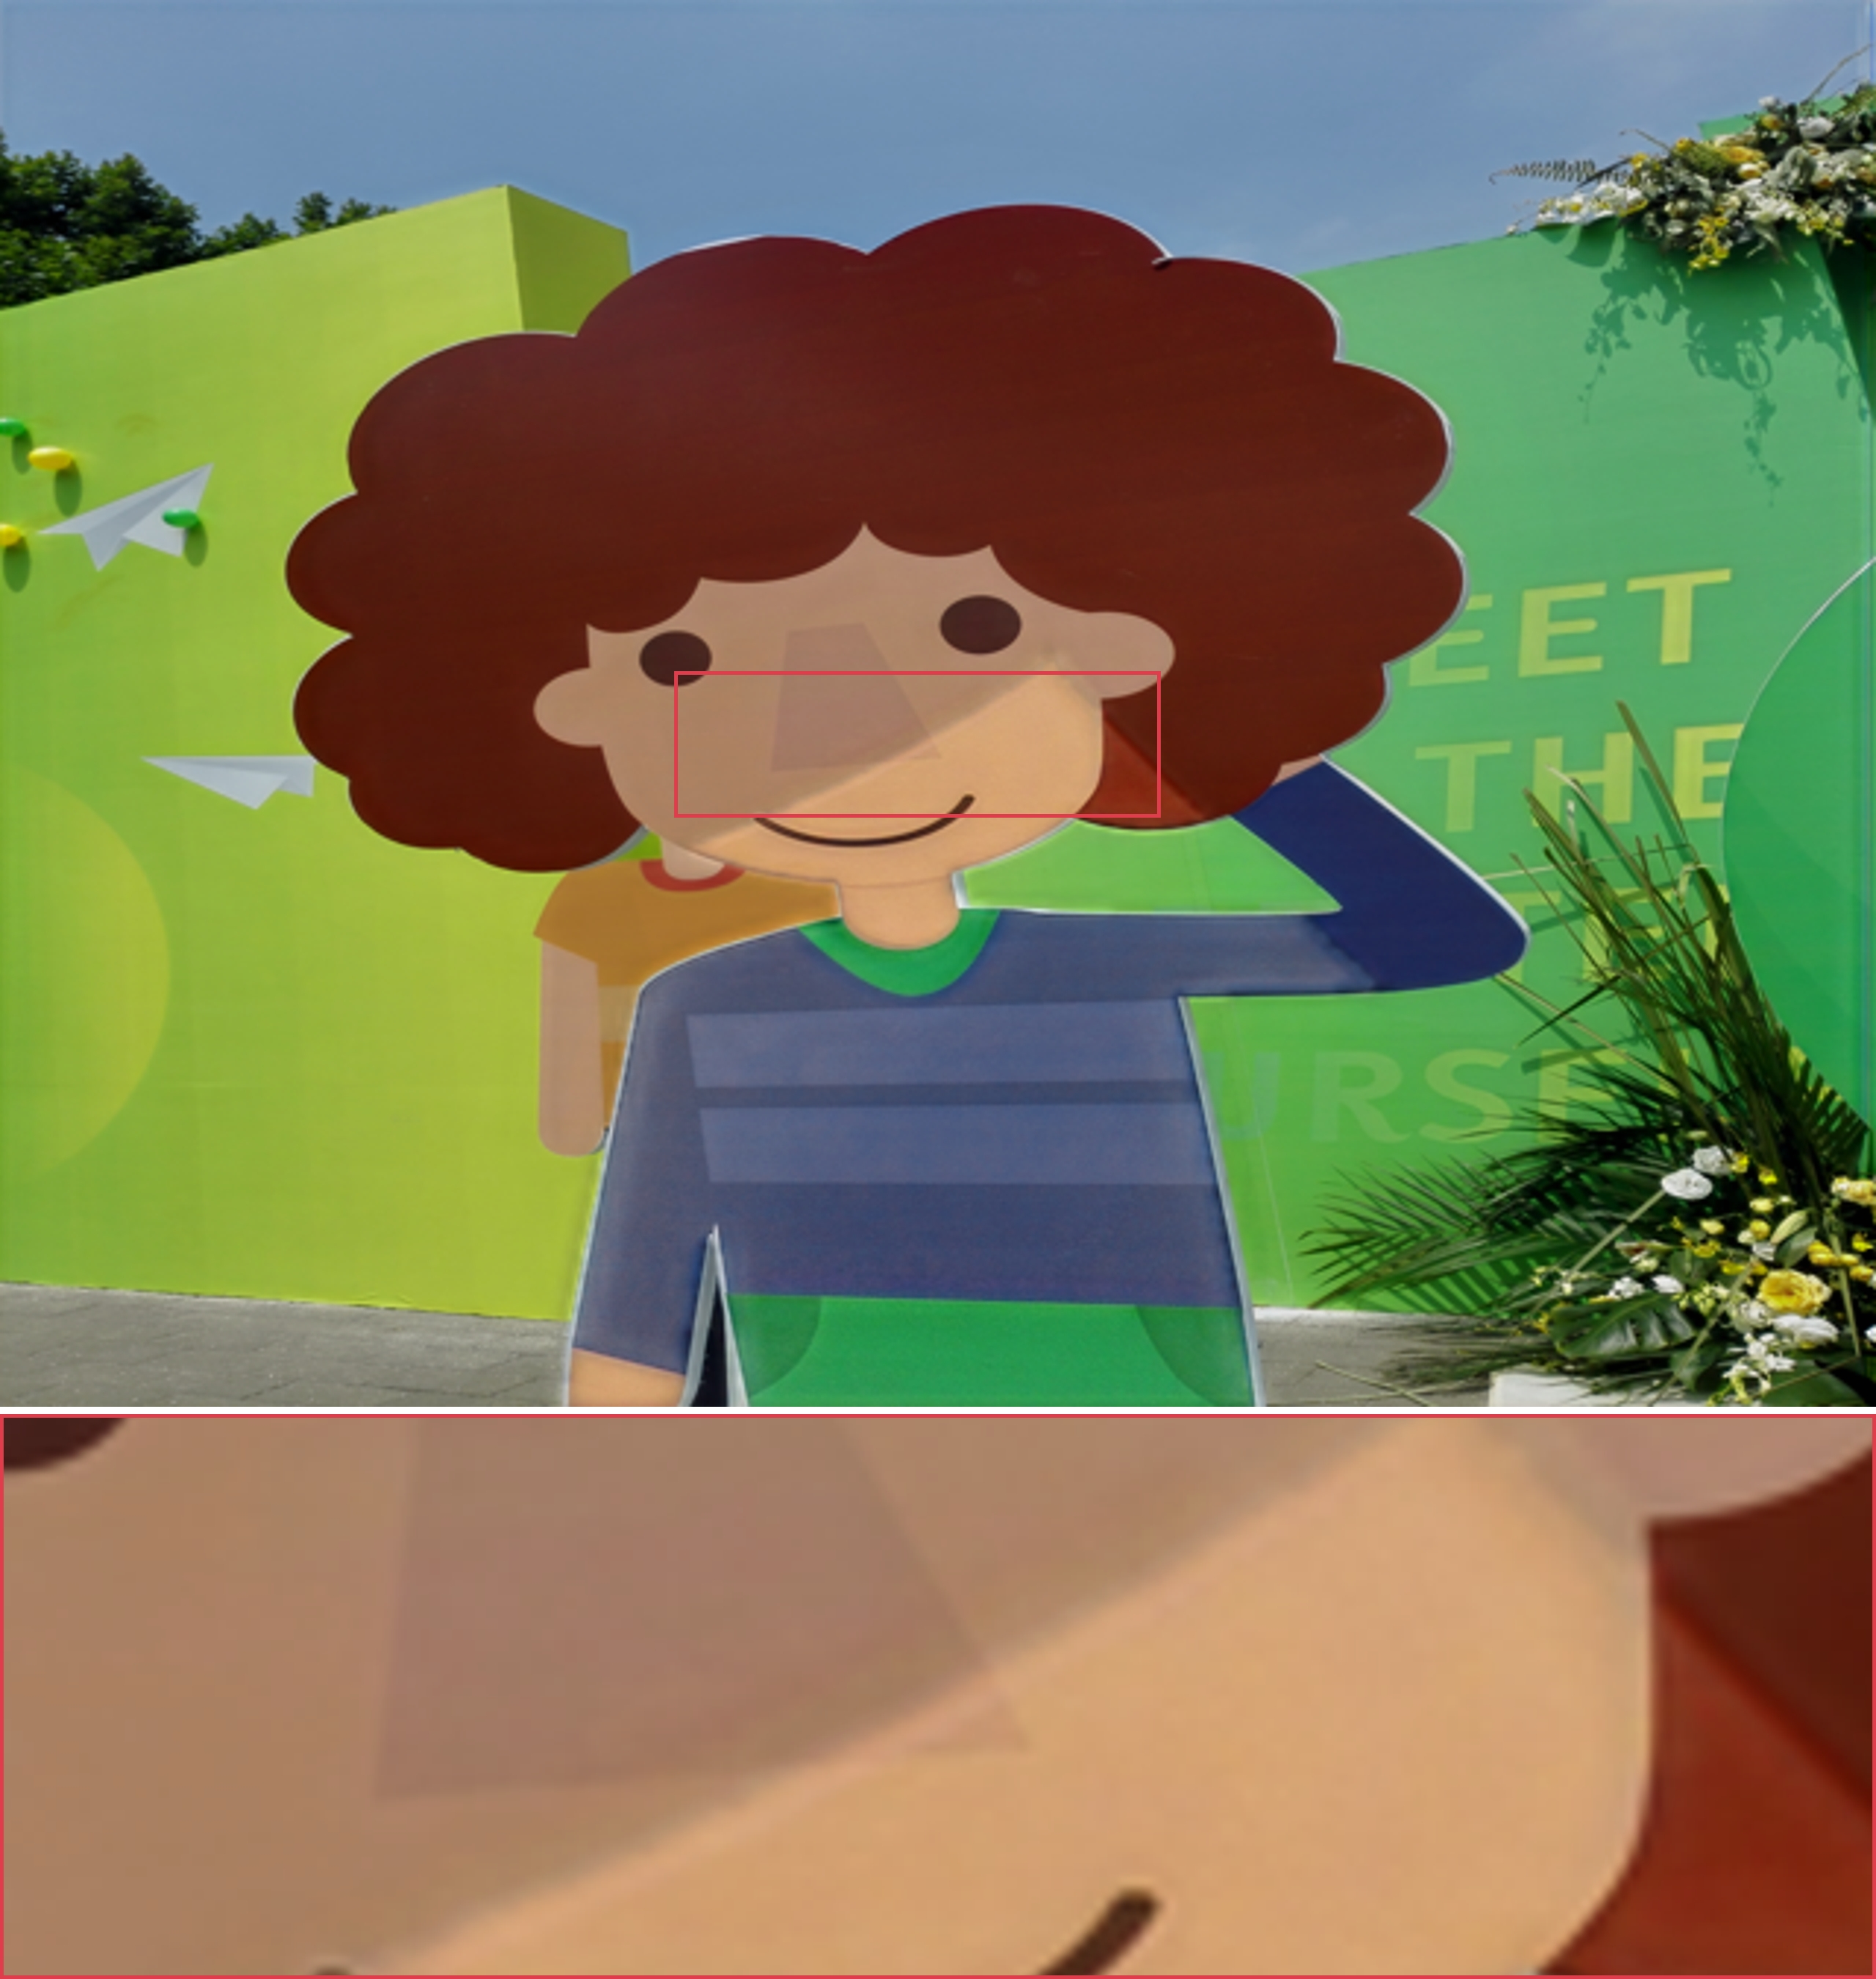}
    \includegraphics[width=.20\linewidth]{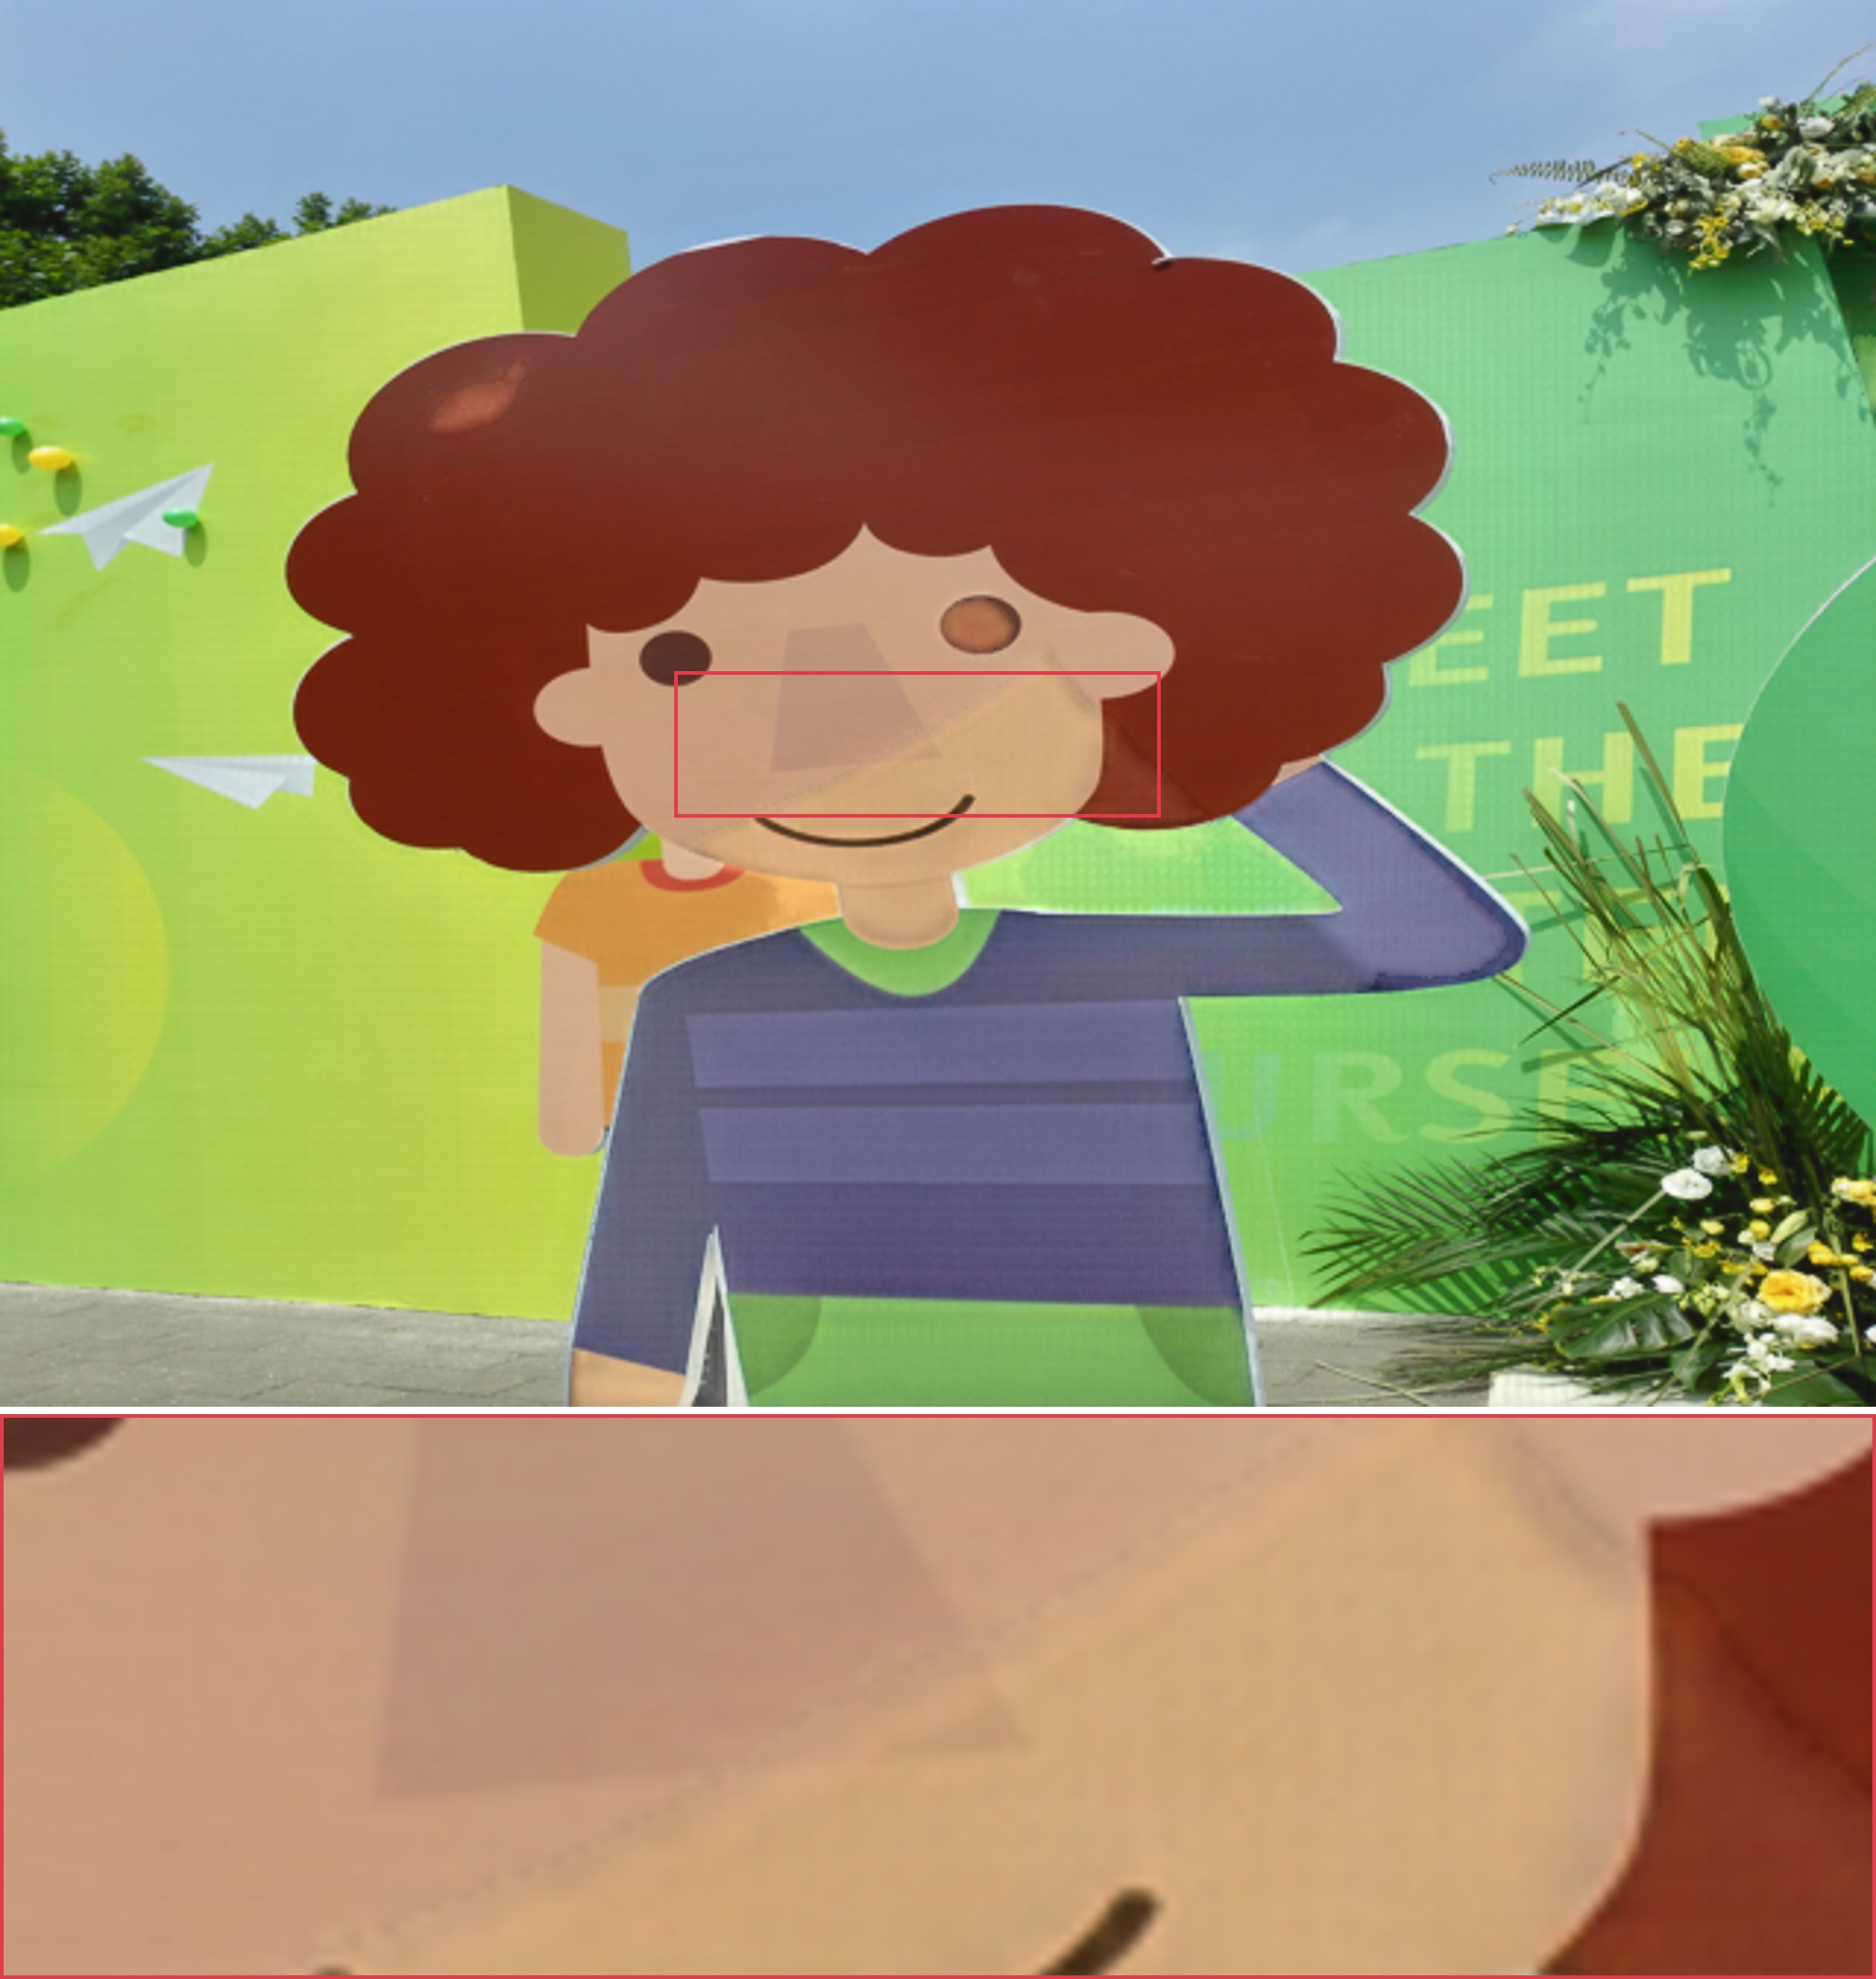}
    \includegraphics[width=.20\linewidth]{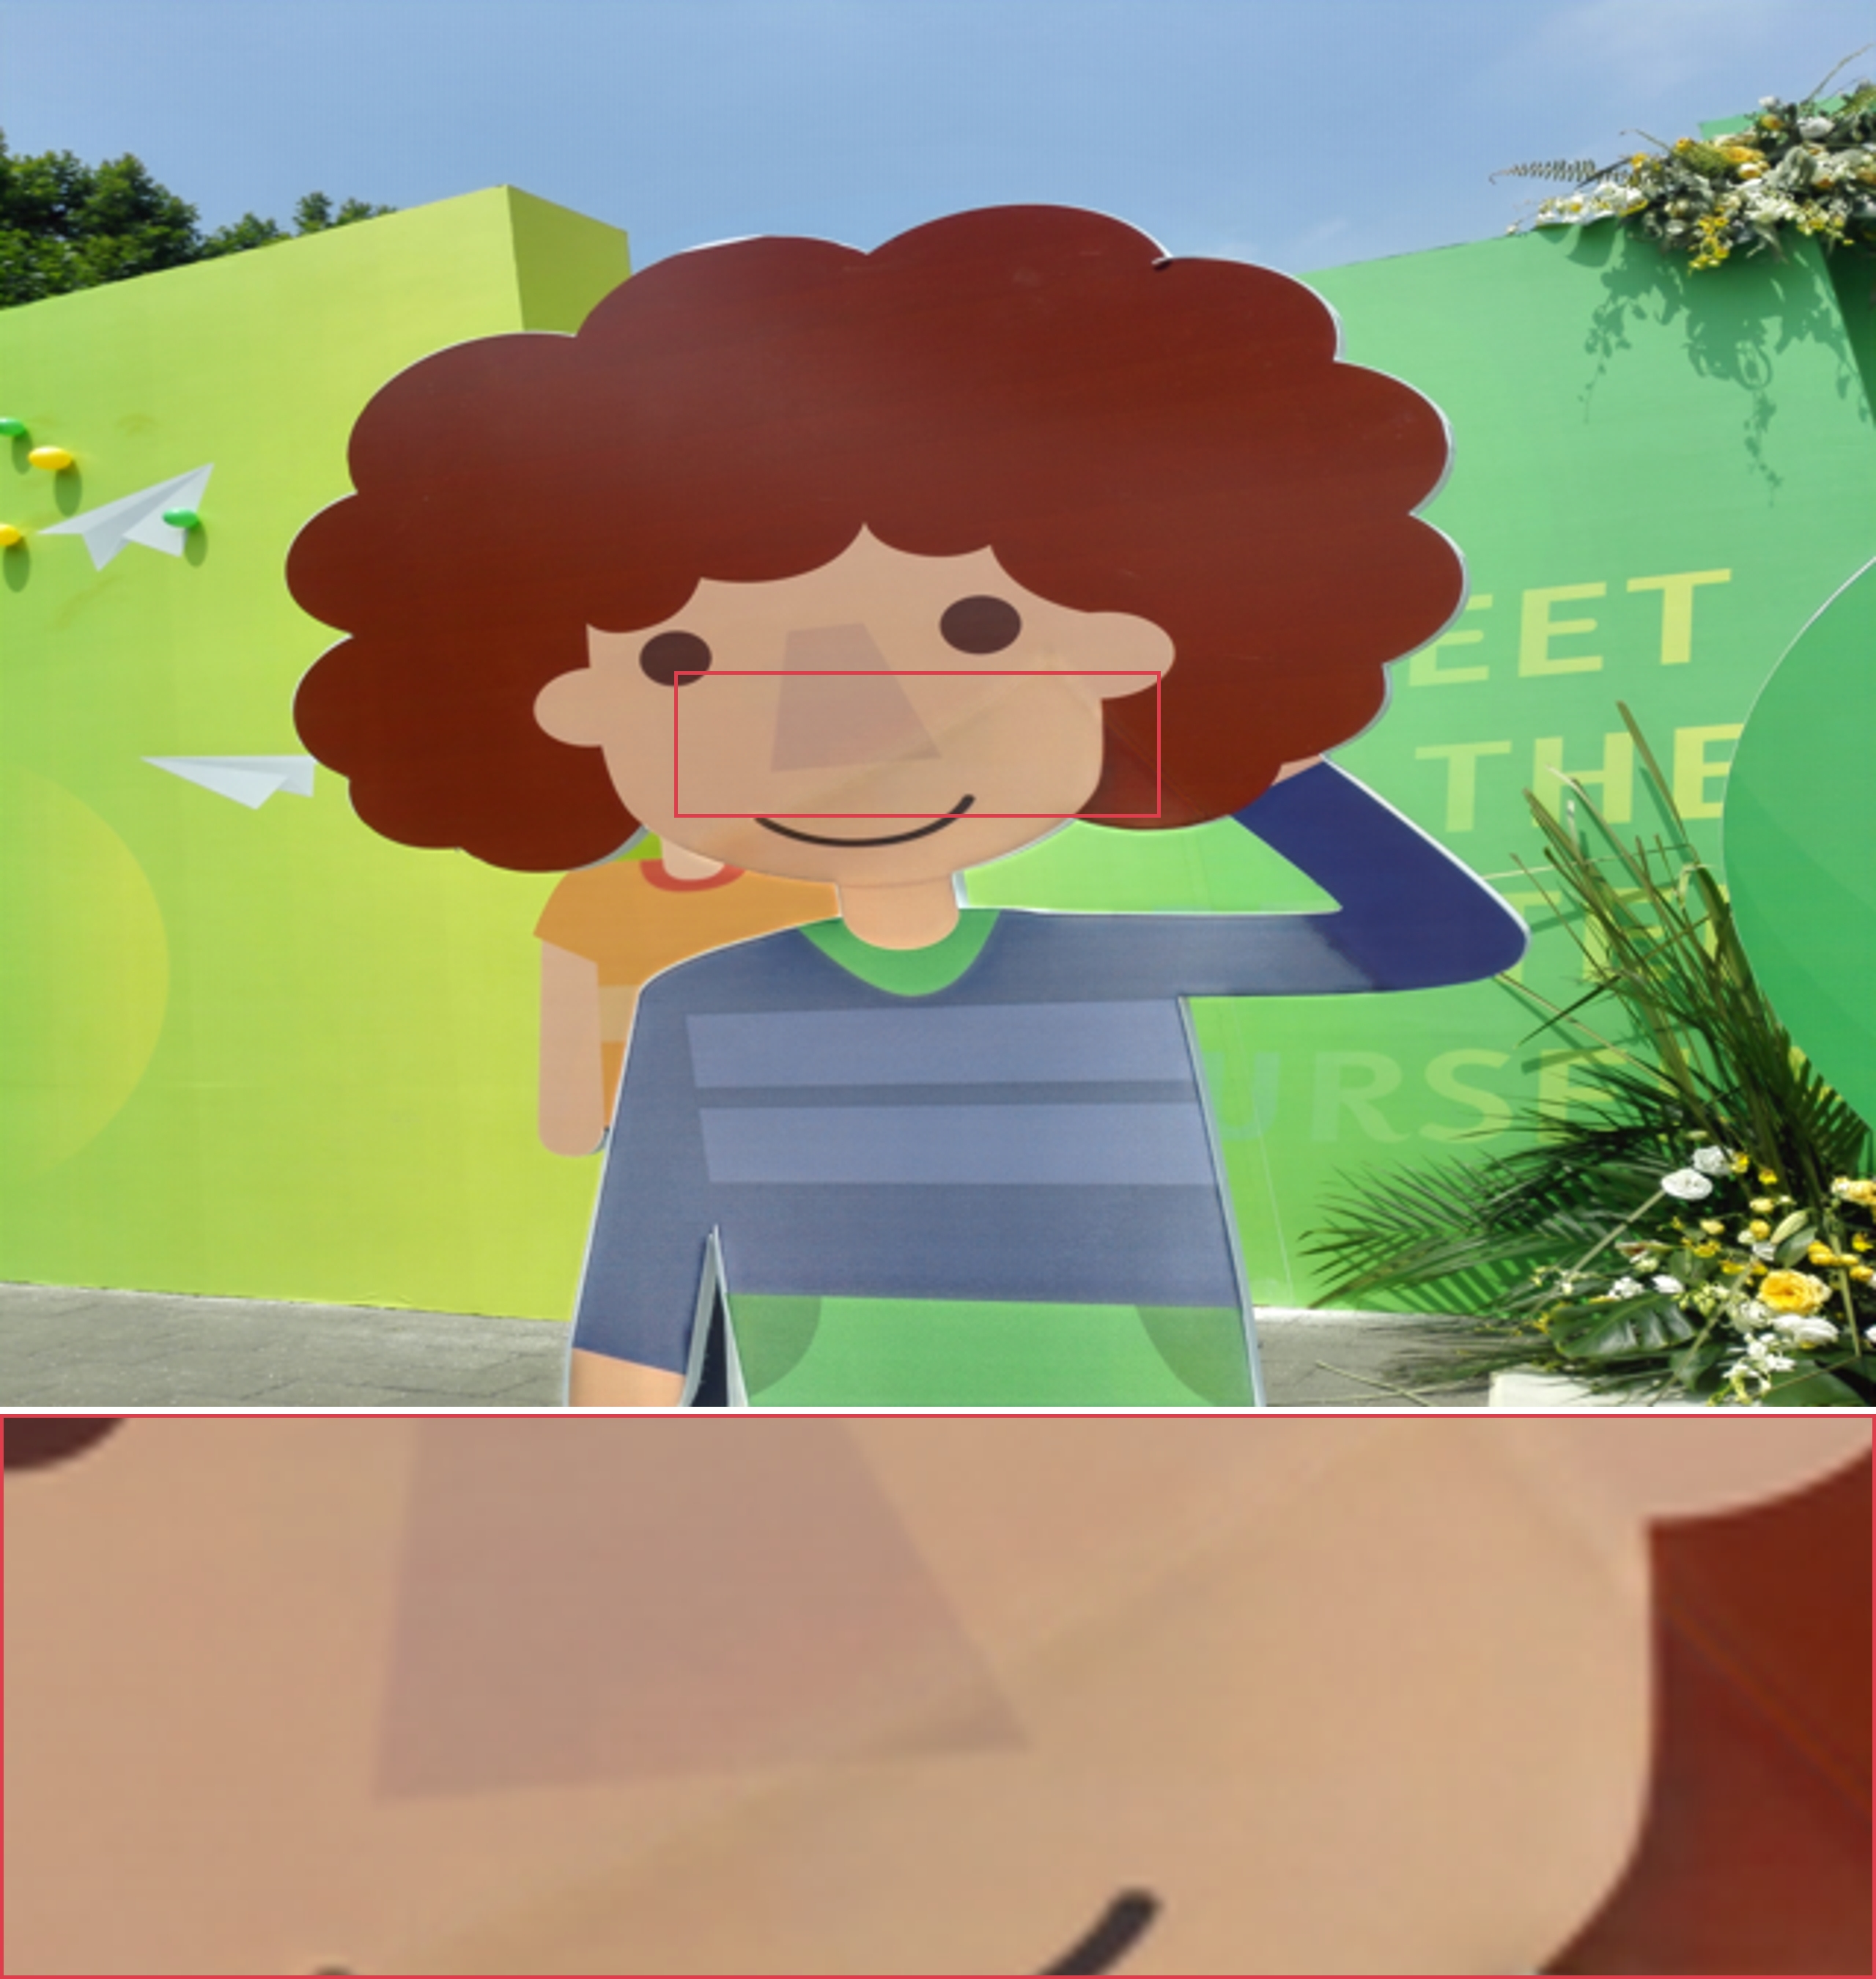}

    \begin{subfigure}{0.20\linewidth}
        \centering
        \subcaption{Input}
    \end{subfigure}
    \begin{subfigure}{0.20\linewidth}
        \centering
        \subcaption{BMNet~\cite{ZhuHFZSZ22}}
    \end{subfigure}
    \begin{subfigure}{0.20\linewidth}
        \centering
        \subcaption{SG~\cite{WanYWWLW22}}
    \end{subfigure}
    \begin{subfigure}{0.20\linewidth}
        \centering
        \subcaption{SF~\cite{GuoHLCW23}}
    \end{subfigure}
    
    \includegraphics[width=.20\linewidth]{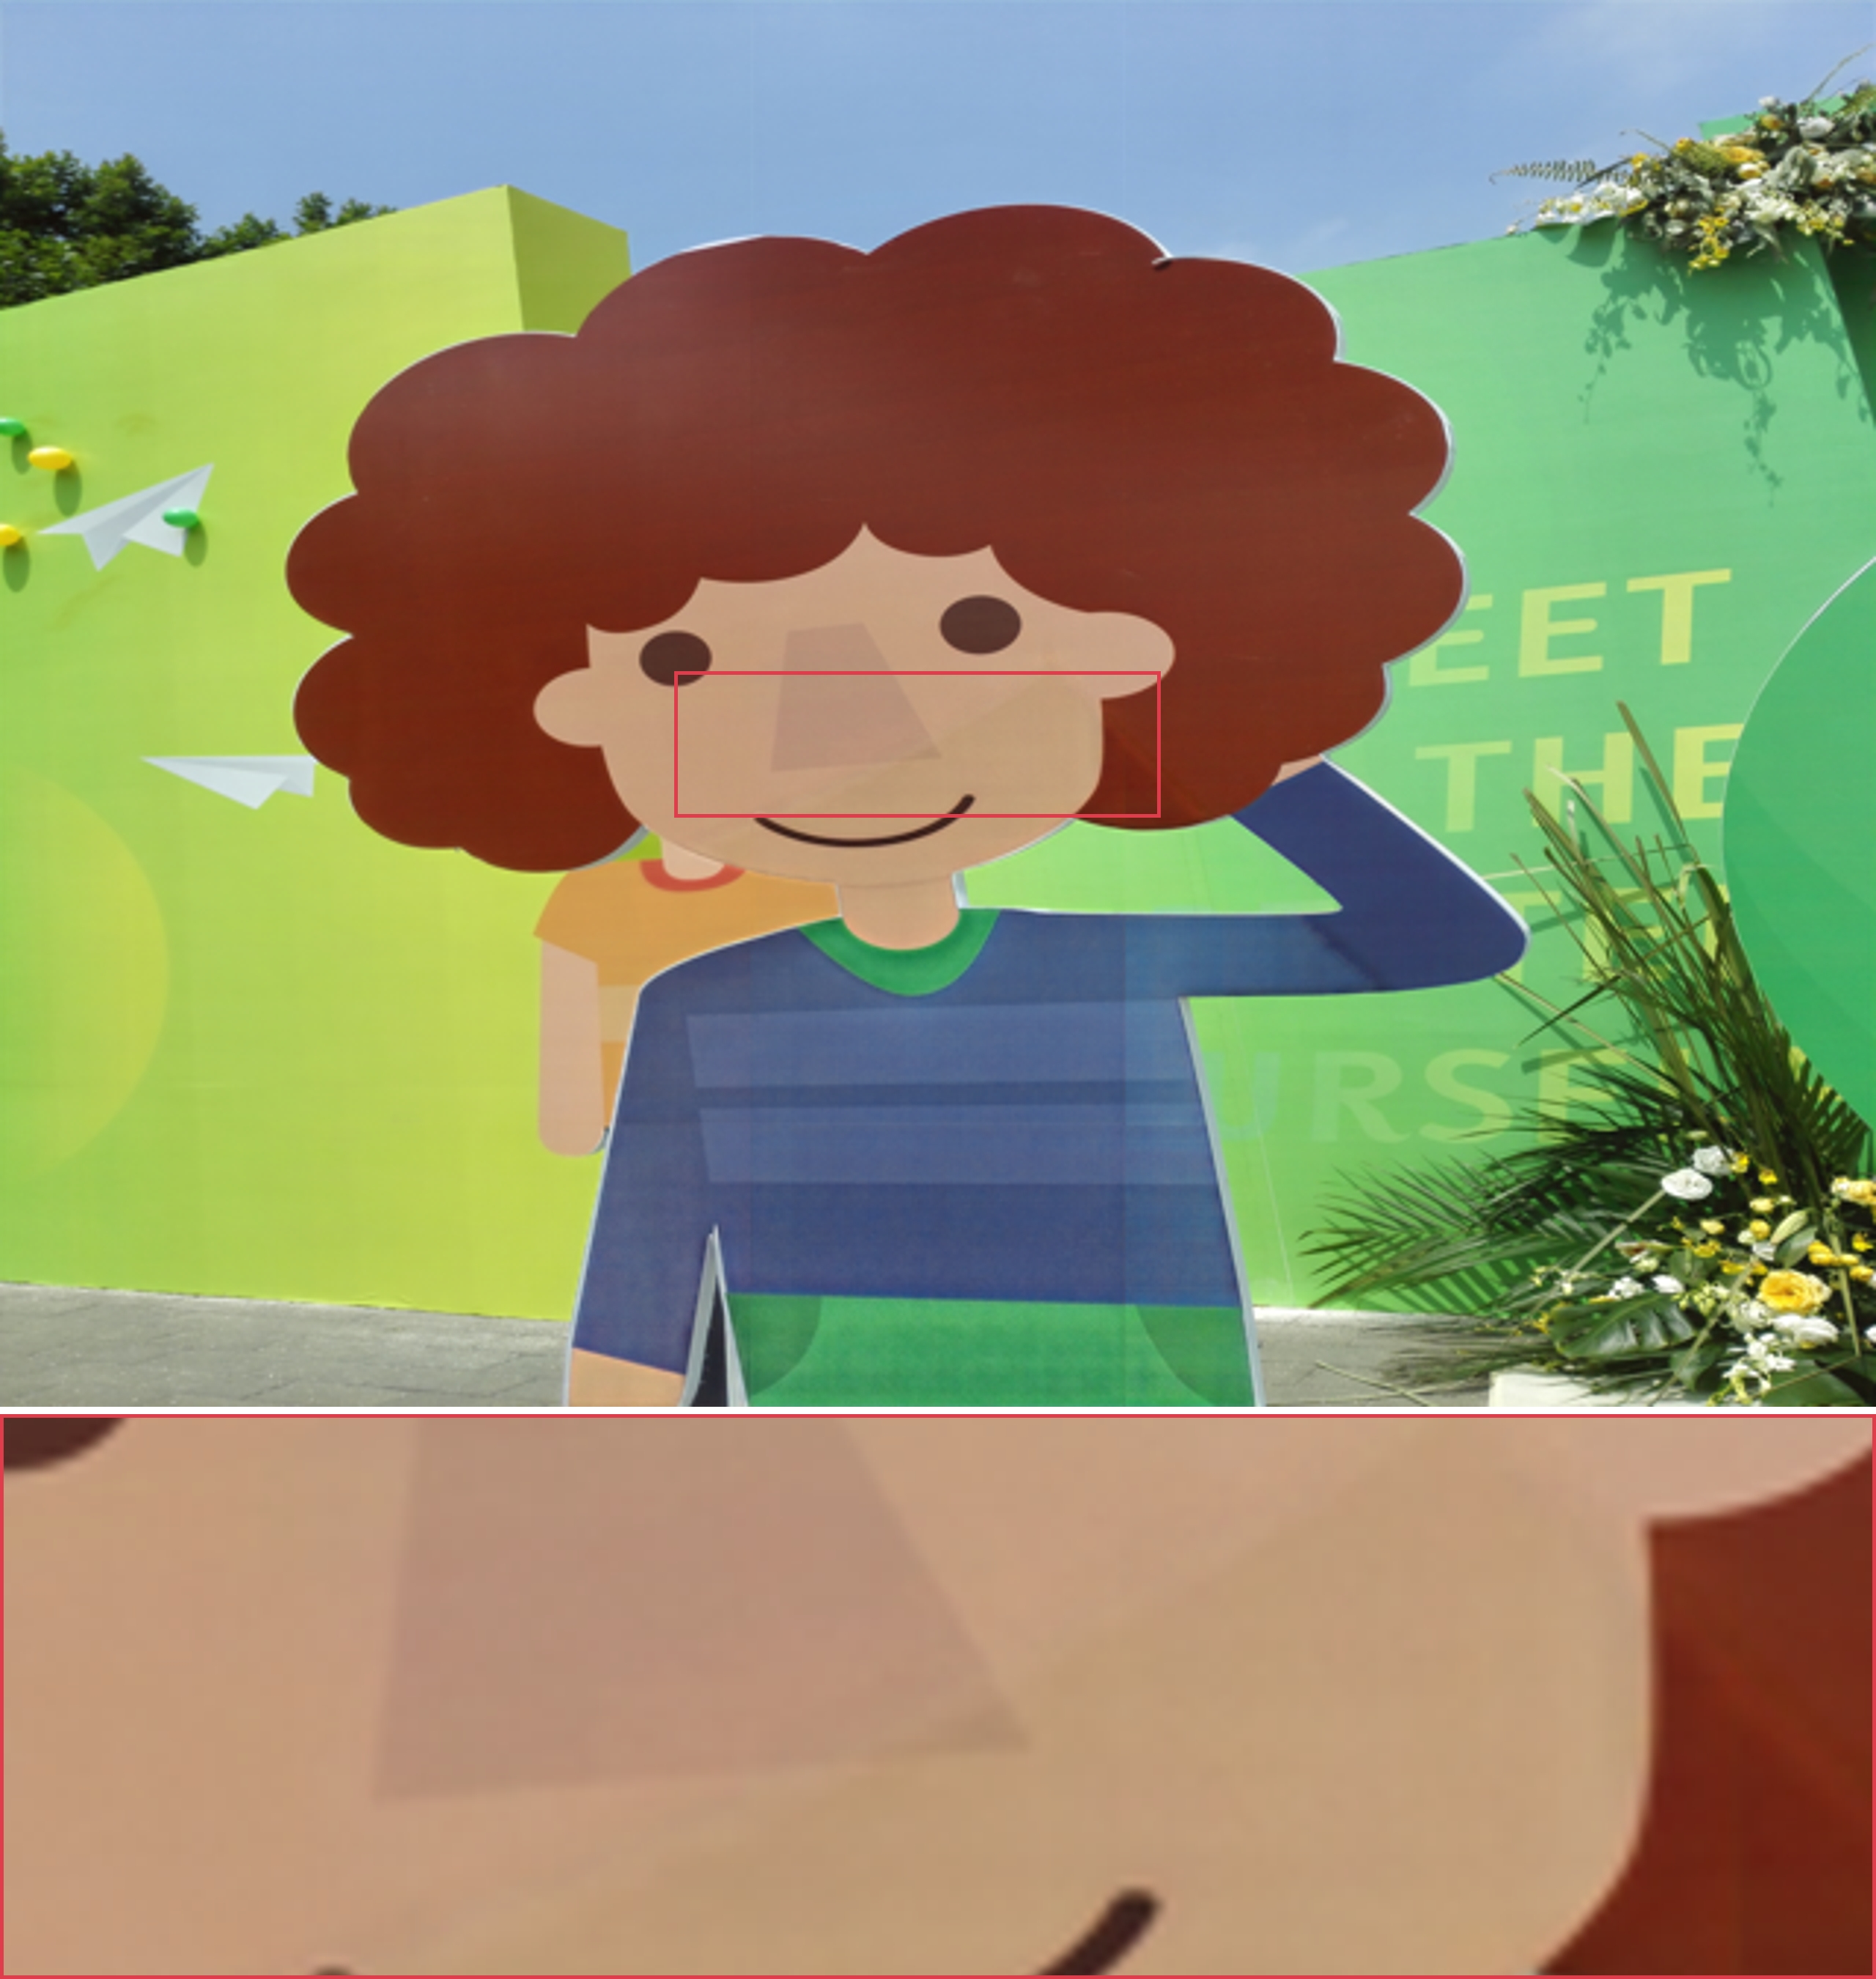}
    \includegraphics[width=.20\linewidth]{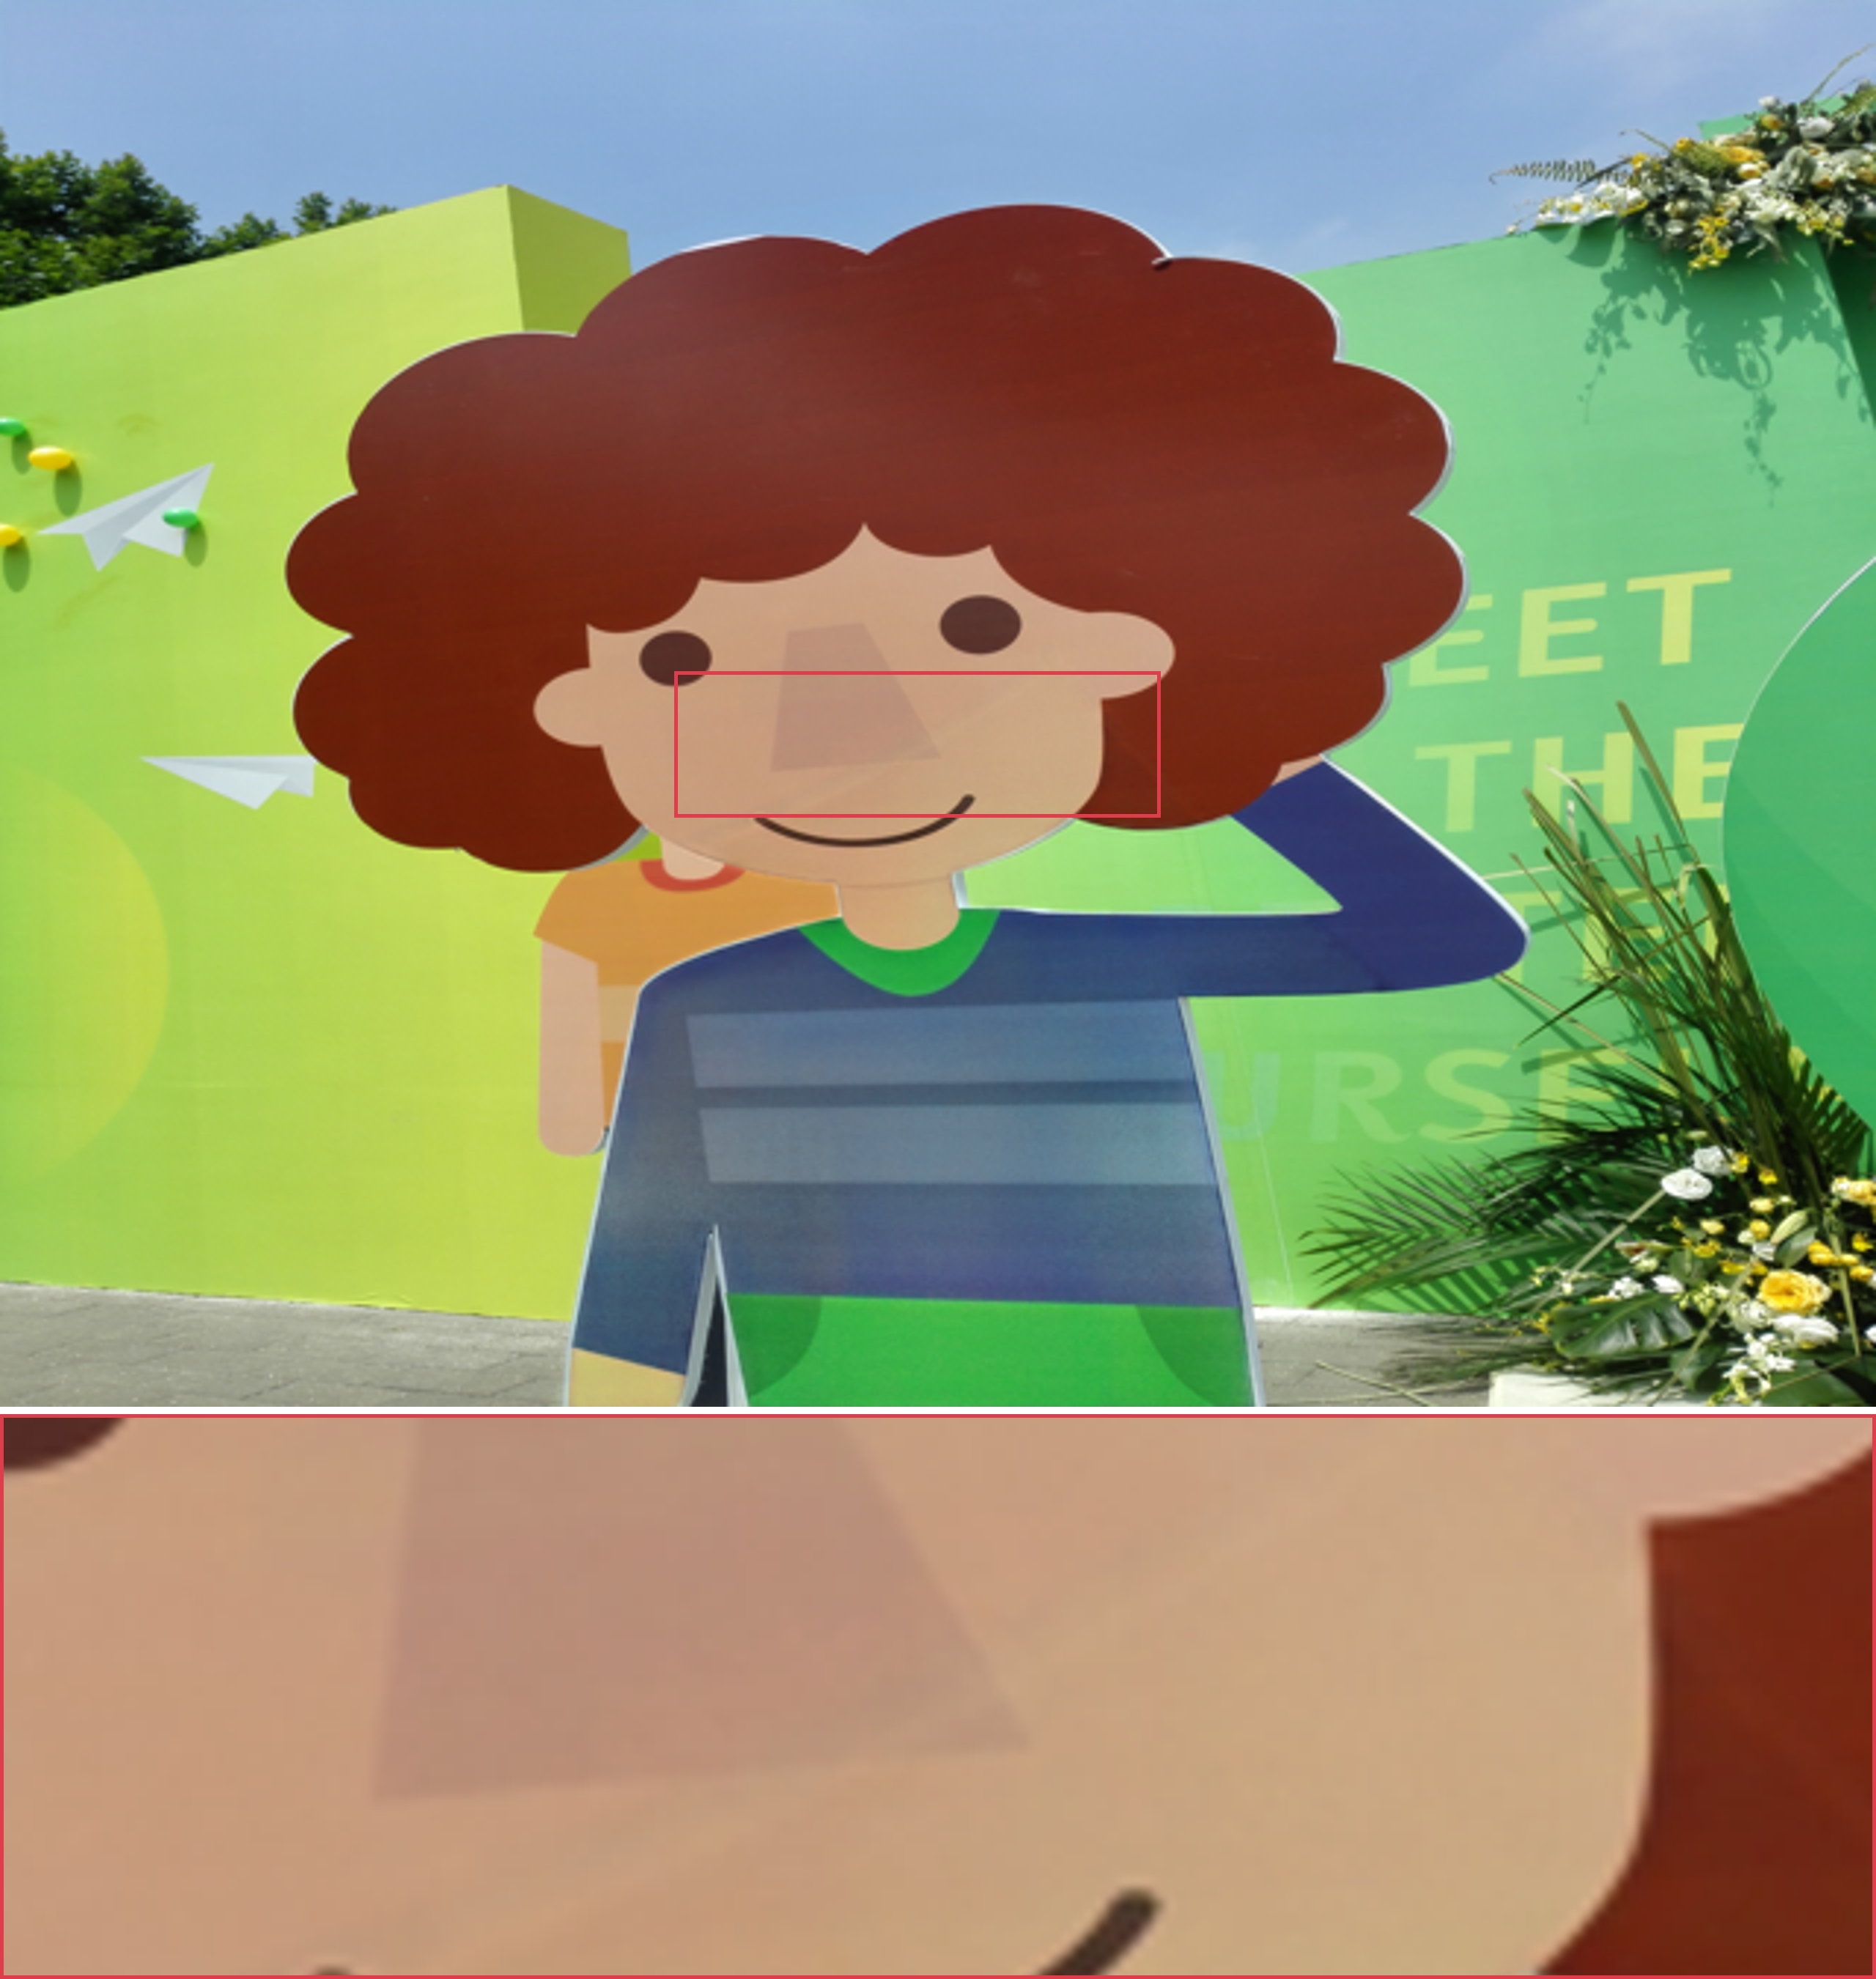}
    \includegraphics[width=.20\linewidth]{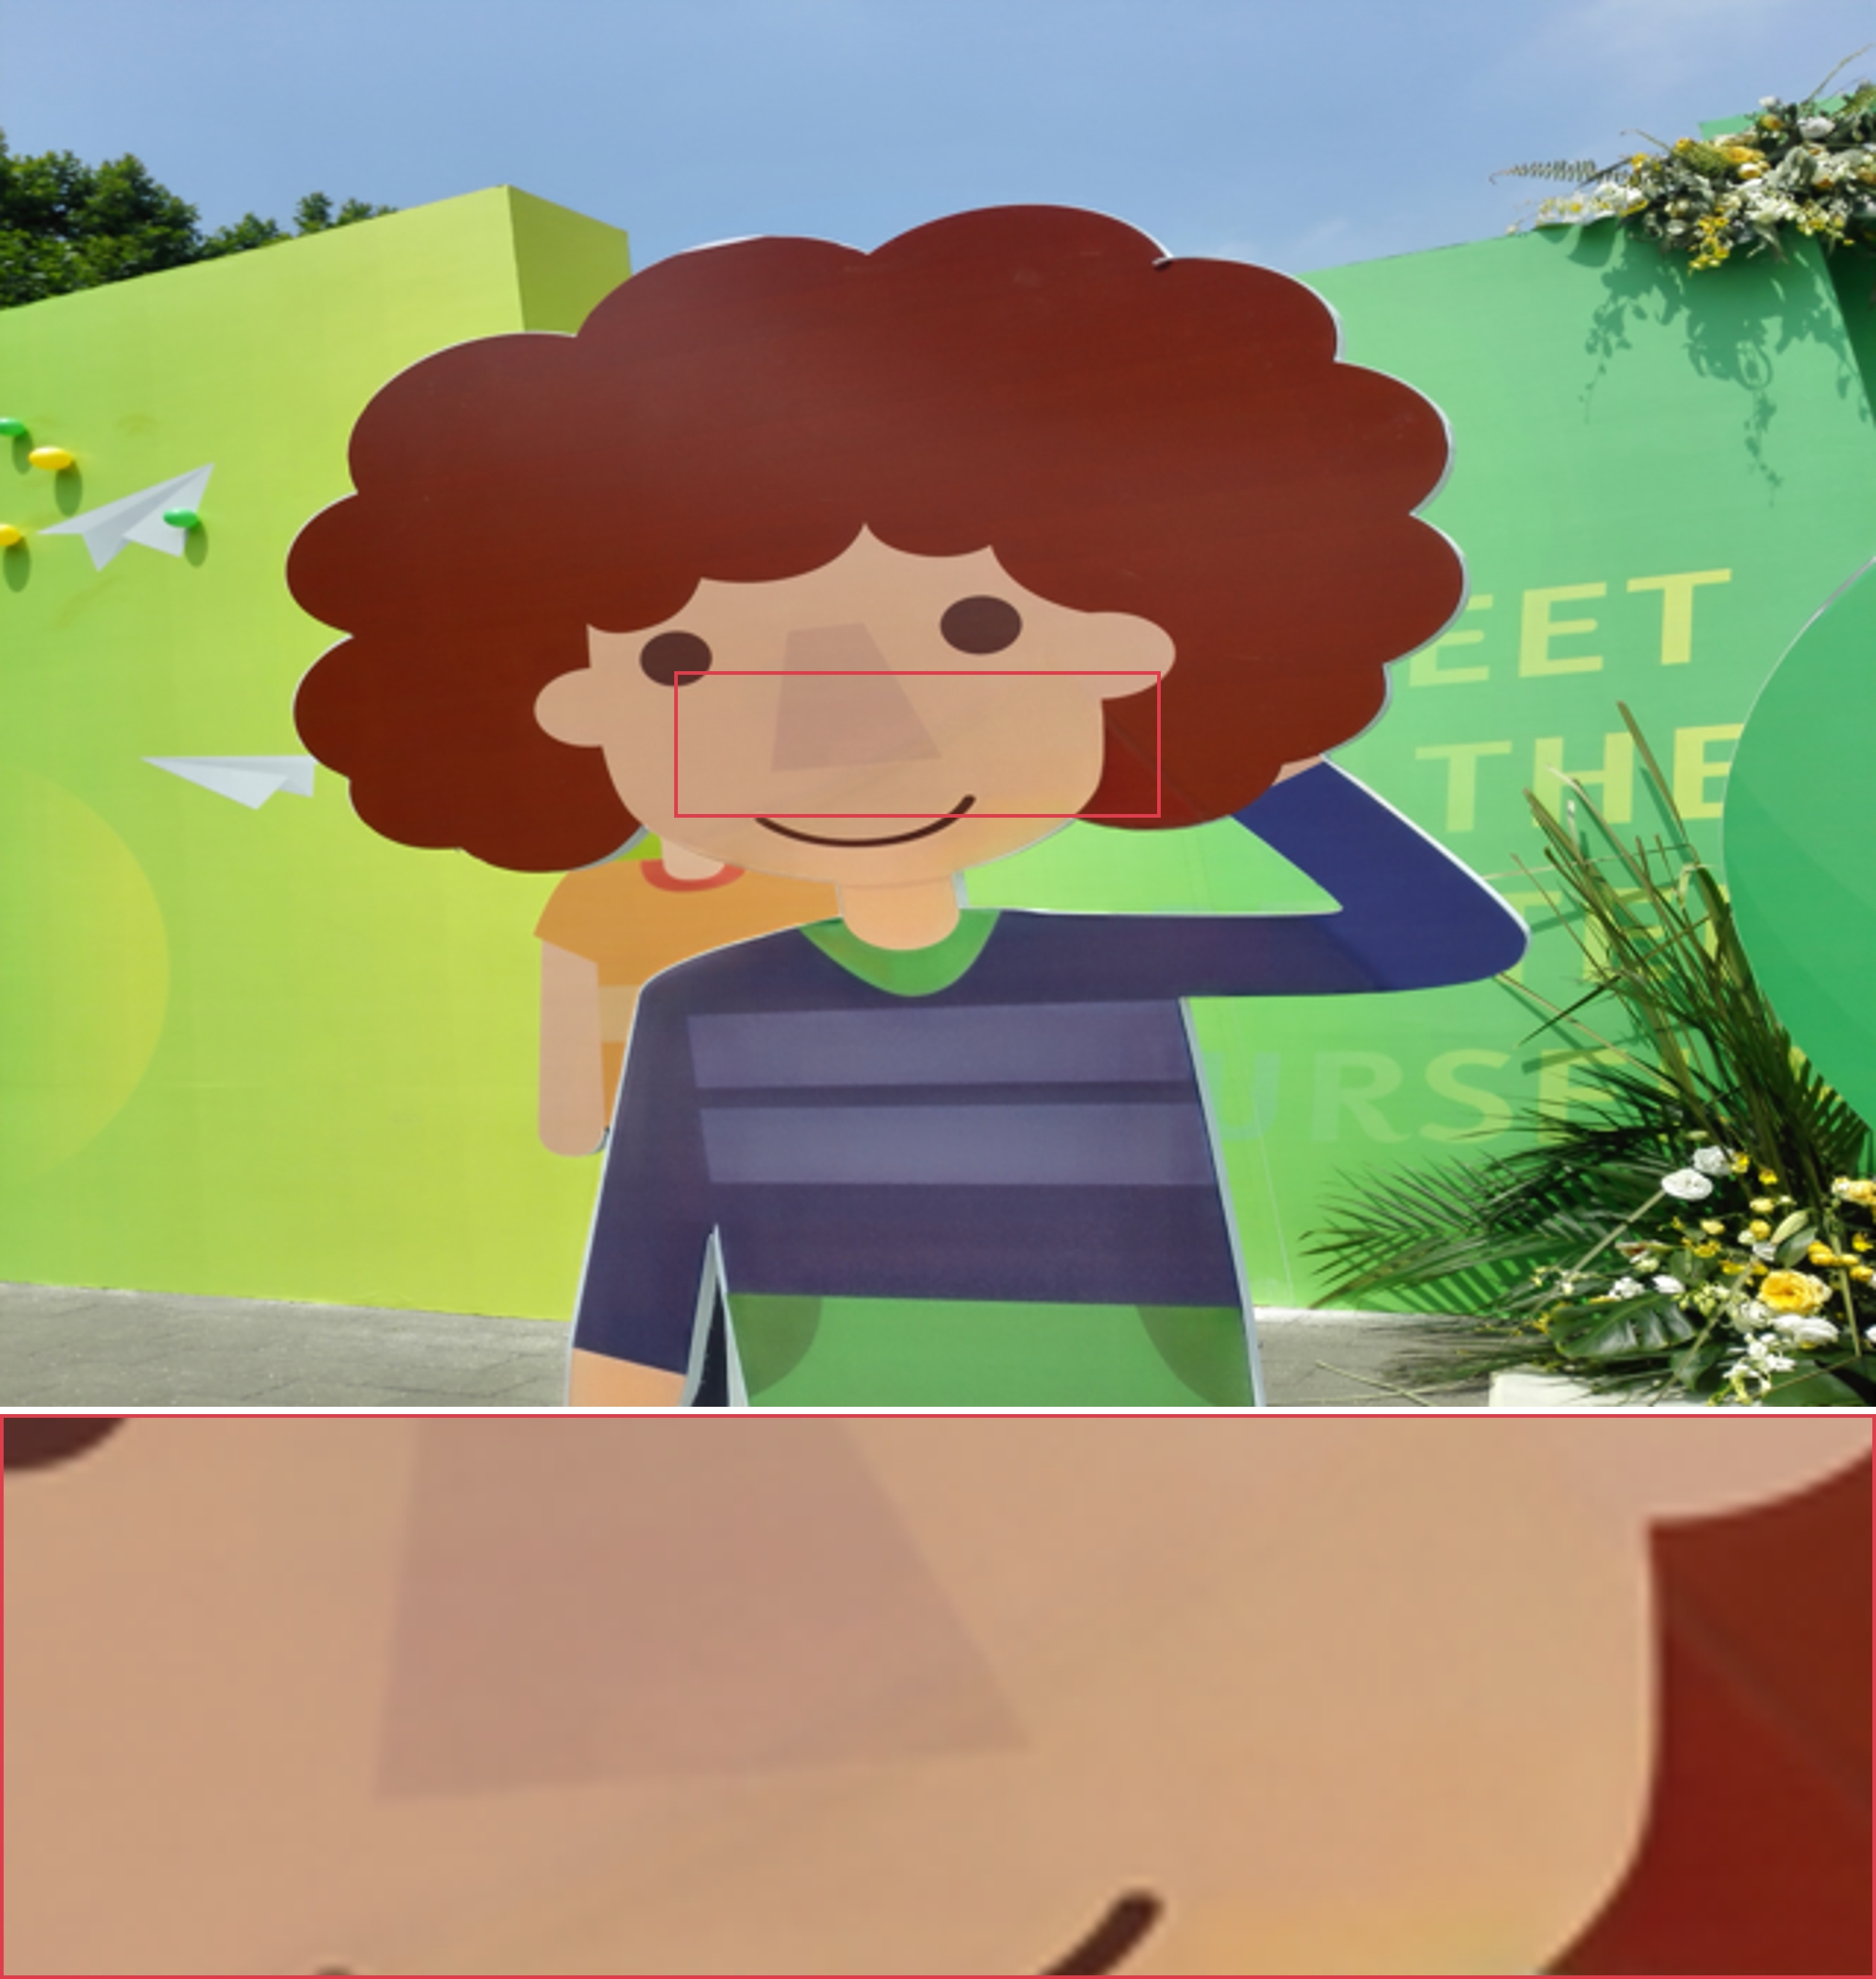}
    \includegraphics[width=.20\linewidth]{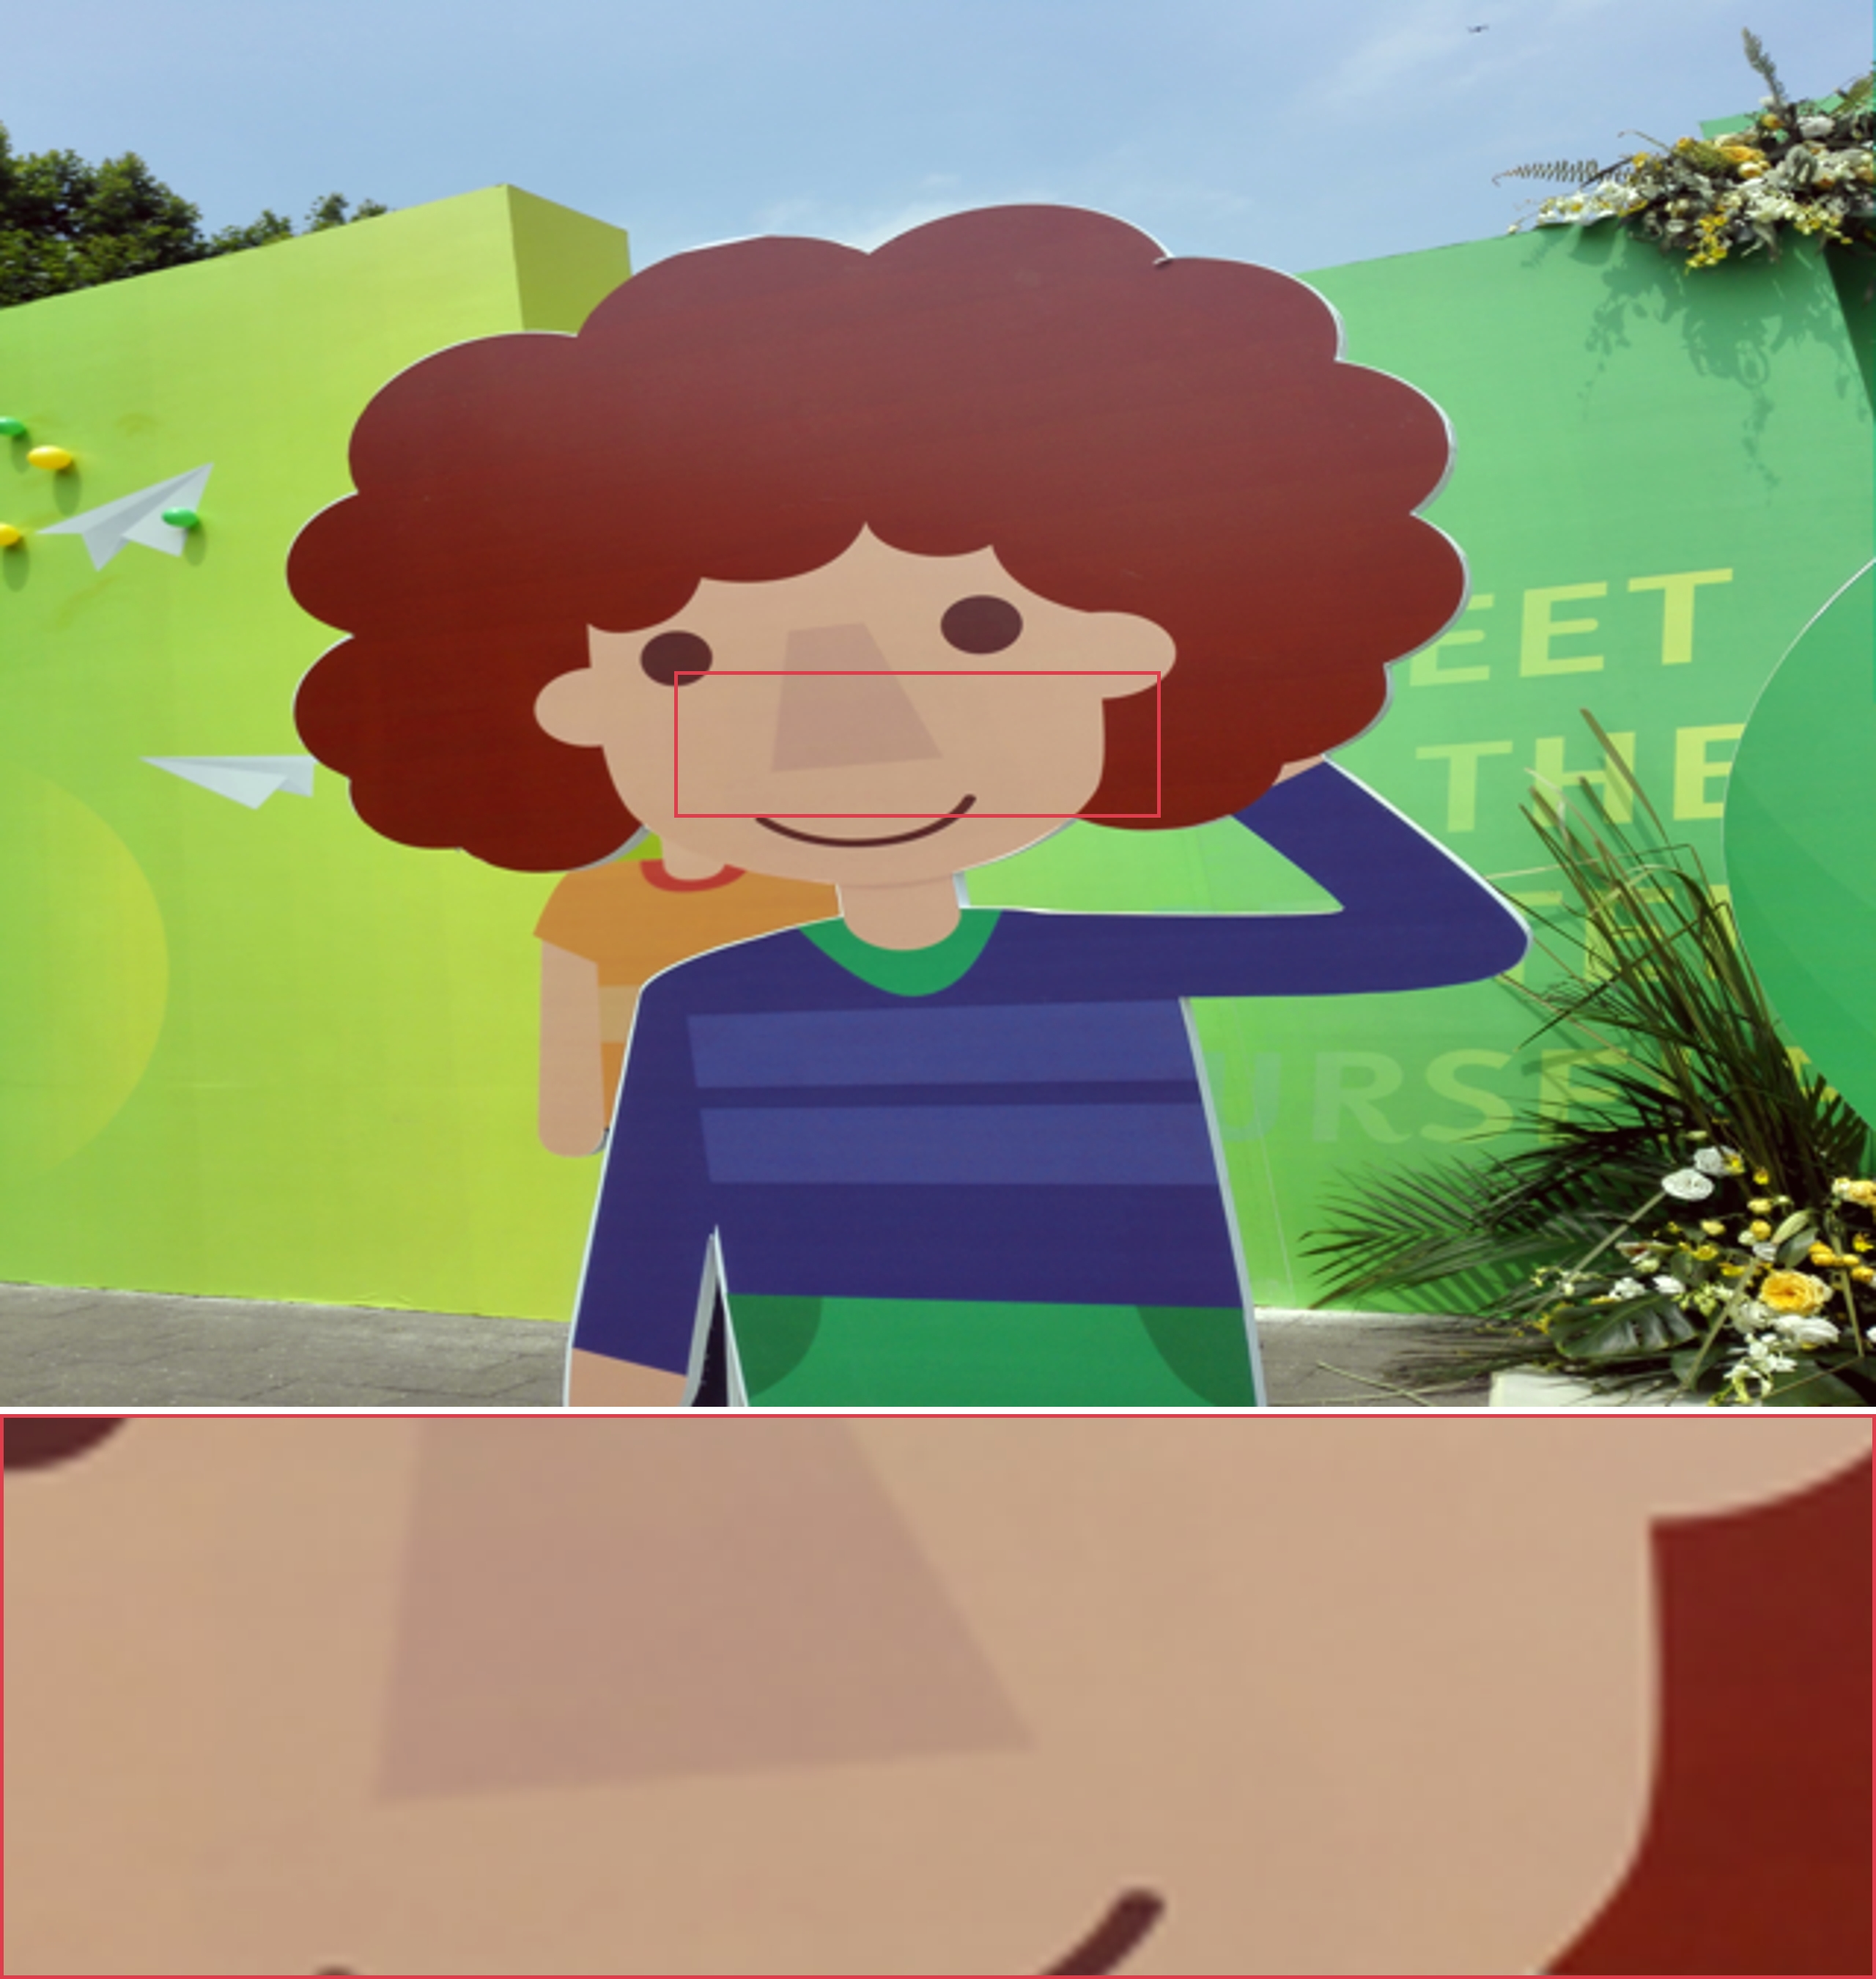}
    
    \begin{subfigure}{0.20\linewidth}
        \centering
        \subcaption{HF~\cite{0002FZL00Z24}}
    \end{subfigure}
    \begin{subfigure}{0.20\linewidth}
        \centering
        \subcaption{RASM~\cite{liu2024regional}}
    \end{subfigure}
    \begin{subfigure}{0.20\linewidth}
        \centering
        \subcaption{Ours}
    \end{subfigure}
    \begin{subfigure}{0.20\linewidth}
        \centering
        \subcaption{GT}
    \end{subfigure}
    
    \vspace{-15pt}
    \caption{Visual comparisons on the ISTD+ dataset. }
    \label{fig:suppl.istd1}
    \vspace{-20pt}
\end{figure*}

\begin{figure*}[t]
    \centering
    \includegraphics[width=.24\linewidth]{fig/4/istd/113/113_113-8-input.jpg}
    \includegraphics[width=.24\linewidth]{fig/4/istd/113/113_113-8-BMNet.jpg}
    \includegraphics[width=.24\linewidth]{fig/4/istd/113/113_113-8-SG.jpg}
    \includegraphics[width=.24\linewidth]{fig/4/istd/113/113_113-8-shadowformer.jpg}

    \begin{subfigure}{0.23\linewidth}
        \centering
        \subcaption{Input}
    \end{subfigure}
    \begin{subfigure}{0.23\linewidth}
        \centering
        \subcaption{BMNet~\cite{ZhuHFZSZ22}}
    \end{subfigure}
    \begin{subfigure}{0.23\linewidth}
        \centering
        \subcaption{SG~\cite{WanYWWLW22}}
    \end{subfigure}
    \begin{subfigure}{0.23\linewidth}
        \centering
        \subcaption{SF~\cite{GuoHLCW23}}
    \end{subfigure}
    
    \includegraphics[width=.24\linewidth]{fig/4/istd/113/113_113-8-homo.jpg}
    \includegraphics[width=.24\linewidth]{fig/4/istd/113/113_113-8-rasm.jpg}
    \includegraphics[width=.24\linewidth]{fig/4/istd/113/113_113-8-ours.jpg}
    \includegraphics[width=.24\linewidth]{fig/4/istd/113/113_113-8-gt.jpg}
    
    \begin{subfigure}{0.23\linewidth}
        \centering
        \subcaption{HF~\cite{0002FZL00Z24}}
    \end{subfigure}
    \begin{subfigure}{0.23\linewidth}
        \centering
        \subcaption{RASM~\cite{liu2024regional}}
    \end{subfigure}
    \begin{subfigure}{0.23\linewidth}
        \centering
        \subcaption{Ours}
    \end{subfigure}
    \begin{subfigure}{0.23\linewidth}
        \centering
        \subcaption{GT}
    \end{subfigure}

    \includegraphics[width=.24\linewidth]{fig/4/istd/96/96-1-input.jpg}
    \includegraphics[width=.24\linewidth]{fig/4/istd/96/96-1-BMNet.jpg}
    \includegraphics[width=.24\linewidth]{fig/4/istd/96/96-1-SG.jpg}
    \includegraphics[width=.24\linewidth]{fig/4/istd/96/96-1-SF.jpg}

    \begin{subfigure}{0.23\linewidth}
        \centering
        \subcaption{Input}
    \end{subfigure}
    \begin{subfigure}{0.23\linewidth}
        \centering
        \subcaption{BMNet~\cite{ZhuHFZSZ22}}
    \end{subfigure}
    \begin{subfigure}{0.23\linewidth}
        \centering
        \subcaption{SG~\cite{WanYWWLW22}}
    \end{subfigure}
    \begin{subfigure}{0.23\linewidth}
        \centering
        \subcaption{SF~\cite{GuoHLCW23}}
    \end{subfigure}
    
    \includegraphics[width=.24\linewidth]{fig/4/istd/96/96-1-homo.jpg}
    \includegraphics[width=.24\linewidth]{fig/4/istd/96/96-1-rasm.jpg}
    \includegraphics[width=.24\linewidth]{fig/4/istd/96/96-1-ours.jpg}
    \includegraphics[width=.24\linewidth]{fig/4/istd/96/96-1-gt.jpg}
    
    \begin{subfigure}{0.23\linewidth}
        \centering
        \subcaption{HF~\cite{0002FZL00Z24}}
    \end{subfigure}
    \begin{subfigure}{0.23\linewidth}
        \centering
        \subcaption{RASM~\cite{liu2024regional}}
    \end{subfigure}
    \begin{subfigure}{0.23\linewidth}
        \centering
        \subcaption{Ours}
    \end{subfigure}
    \begin{subfigure}{0.23\linewidth}
        \centering
        \subcaption{GT}
    \end{subfigure}

    \vspace{15pt}\caption{Visual comparisons on the ISTD+ dataset. }
    \label{fig:suppl.istd2}
        \vspace{20pt}
\end{figure*}
We display more visual comparisons on the ISTD+~\cite{LeS19} and SRD~\cite{QuTHTL17} datasets in Figs.~\ref{fig:suppl.istd1}, \ref{fig:suppl.istd2}, \ref{fig:suppl.srd1} and \ref{fig:suppl.srd2}. Additionally, Fig~\ref{fig:suppl.ucfuiuc} brings extra UIUC and UCF datasets results.

\begin{figure*}[t]
    \centering
    
    \includegraphics[width=.24\linewidth]{fig/4/srd/2437/_MG_2437__MG_2437_input-_MG_2437__MG_2437_input.jpg}
    \includegraphics[width=.24\linewidth]{fig/4/srd/2437/_MG_2437__MG_2437_BMNet-_MG_2437__MG_2437_BMNet.jpg}
    \includegraphics[width=.24\linewidth]{fig/4/srd/2437/_MG_2437__MG_2437_sg-_MG_2437__MG_2437_sg.jpg}
    \includegraphics[width=.24\linewidth]{fig/4/srd/2437/_MG_2437__MG_2437_DMTN-_MG_2437__MG_2437_DMTN.jpg}

    \begin{subfigure}{0.23\linewidth}
        \centering
        \subcaption{Input}
    \end{subfigure}
    \begin{subfigure}{0.23\linewidth}
        \centering
        \subcaption{BMNet~\cite{ZhuHFZSZ22}}
    \end{subfigure}
    \begin{subfigure}{0.23\linewidth}
        \centering
        \subcaption{SG~\cite{WanYWWLW22}}
    \end{subfigure}
        \begin{subfigure}{0.23\linewidth}
        \centering
        \subcaption{DMTN~\cite{LiuWFLQT23}}
    \end{subfigure}
    
    \includegraphics[width=.24\linewidth]{fig/4/srd/2437/_MG_2437__MG_2437_des3-_MG_2437__MG_2437_des3.jpg}
    \includegraphics[width=.24\linewidth]{fig/4/srd/2437/_MG_2437__MG_2437_homo-_MG_2437__MG_2437_homo.jpg}
    \includegraphics[width=.24\linewidth]{fig/4/srd/2437/_MG_2437__MG_2437_ours-_MG_2437__MG_2437_ours.jpg}
    \includegraphics[width=.24\linewidth]{fig/4/srd/2437/_MG_2437__MG_2437_gt-_MG_2437__MG_2437_gt.jpg}

    \begin{subfigure}{0.23\linewidth}
        \centering
        \subcaption{DeS3~\cite{Jin0YYT24}}
    \end{subfigure}
    \begin{subfigure}{0.23\linewidth}
        \centering
        \subcaption{HF~\cite{0002FZL00Z24}}
    \end{subfigure}
    \begin{subfigure}{0.23\linewidth}
        \centering
        \subcaption{Ours}
    \end{subfigure}
    \begin{subfigure}{0.23\linewidth}
        \centering
        \subcaption{GT}
    \end{subfigure}
    
    \includegraphics[width=.24\linewidth]{fig/4/srd/2445/_MG_2445__MG_2445_input-_MG_2445__MG_2445_input.jpg}
    \includegraphics[width=.24\linewidth]{fig/4/srd/2445/_MG_2445__MG_2445_BMNet-_MG_2445__MG_2445_BMNet.jpg}
    \includegraphics[width=.24\linewidth]{fig/4/srd/2445/_MG_2445__MG_2445_sg-_MG_2445__MG_2445_sg.jpg}
    \includegraphics[width=.24\linewidth]{fig/4/srd/2445/_MG_2445__MG_2445_DMTN-_MG_2445__MG_2445_DMTN.jpg}

    \begin{subfigure}{0.23\linewidth}
        \centering
        \subcaption{Input}
    \end{subfigure}
    \begin{subfigure}{0.23\linewidth}
        \centering
        \subcaption{BMNet~\cite{ZhuHFZSZ22}}
    \end{subfigure}
    \begin{subfigure}{0.23\linewidth}
        \centering
        \subcaption{SG~\cite{WanYWWLW22}}
    \end{subfigure}
        \begin{subfigure}{0.23\linewidth}
        \centering
        \subcaption{DMTN~\cite{LiuWFLQT23}}
    \end{subfigure}
    
    \includegraphics[width=.24\linewidth]{fig/4/srd/2445/_MG_2445__MG_2445_des3-_MG_2445__MG_2445_des3.jpg}
    \includegraphics[width=.24\linewidth]{fig/4/srd/2445/_MG_2445__MG_2445_homo-_MG_2445__MG_2445_homo.jpg}
    \includegraphics[width=.24\linewidth]{fig/4/srd/2445/_MG_2445__MG_2445_ours-_MG_2445__MG_2445_ours.jpg}
    \includegraphics[width=.24\linewidth]{fig/4/srd/2445/_MG_2445__MG_2445_gt-_MG_2445__MG_2445_gt.jpg}

    \begin{subfigure}{0.23\linewidth}
        \centering
        \subcaption{DeS3~\cite{Jin0YYT24}}
    \end{subfigure}
    \begin{subfigure}{0.23\linewidth}
        \centering
        \subcaption{HF~\cite{0002FZL00Z24}}
    \end{subfigure}
    \begin{subfigure}{0.23\linewidth}
        \centering
        \subcaption{Ours}
    \end{subfigure}
    \begin{subfigure}{0.23\linewidth}
        \centering
        \subcaption{GT}
    \end{subfigure}
    \caption{Visual comparisons on the SRD dataset. } 
    \label{fig:suppl.srd1}
        % \vspace{20pt}
\end{figure*}

\begin{figure*}[t]
    \centering
    
    \includegraphics[width=.24\linewidth]{fig/4/srd/6573/IMG_6573-input.jpg}
    \includegraphics[width=.24\linewidth]{fig/4/srd/6573/IMG_6573-BMNet.jpg}
    \includegraphics[width=.24\linewidth]{fig/4/srd/6573/IMG_6573-SG.jpg}
    \includegraphics[width=.24\linewidth]{fig/4/srd/6573/IMG_6573-DMTN.jpg}

    \begin{subfigure}{0.23\linewidth}
        \centering
        \subcaption{Input}
    \end{subfigure}
    \begin{subfigure}{0.23\linewidth}
        \centering
        \subcaption{BMNet~\cite{ZhuHFZSZ22}}
    \end{subfigure}
    \begin{subfigure}{0.23\linewidth}
        \centering
        \subcaption{SG~\cite{WanYWWLW22}}
    \end{subfigure}
        \begin{subfigure}{0.23\linewidth}
        \centering
        \subcaption{DMTN~\cite{LiuWFLQT23}}
    \end{subfigure}
    
    \includegraphics[width=.24\linewidth]{fig/4/srd/6573/IMG_6573-des3.jpg}
    \includegraphics[width=.24\linewidth]{fig/4/srd/6573/IMG_6573-homo.jpg}
    \includegraphics[width=.24\linewidth]{fig/4/srd/6573/IMG_6573-ours.jpg}
    \includegraphics[width=.24\linewidth]{fig/4/srd/6573/IMG_6573-gt.jpg}

    \begin{subfigure}{0.23\linewidth}
        \centering
        \subcaption{DeS3~\cite{Jin0YYT24}}
    \end{subfigure}
    \begin{subfigure}{0.23\linewidth}
        \centering
        \subcaption{HF~\cite{0002FZL00Z24}}
    \end{subfigure}
    \begin{subfigure}{0.23\linewidth}
        \centering
        \subcaption{Ours}
    \end{subfigure}
    \begin{subfigure}{0.23\linewidth}
        \centering
        \subcaption{GT}
    \end{subfigure}
    
    \includegraphics[width=.24\linewidth]{fig/4/srd/6651/IMG_6651-input.jpg}
    \includegraphics[width=.24\linewidth]{fig/4/srd/6651/IMG_6651-BMNet.jpg}
    \includegraphics[width=.24\linewidth]{fig/4/srd/6651/IMG_6651-SG.jpg}
    \includegraphics[width=.24\linewidth]{fig/4/srd/6651/IMG_6651-DMTN.jpg}

    \begin{subfigure}{0.23\linewidth}
        \centering
        \subcaption{Input}
    \end{subfigure}
    \begin{subfigure}{0.23\linewidth}
        \centering
        \subcaption{BMNet~\cite{ZhuHFZSZ22}}
    \end{subfigure}
    \begin{subfigure}{0.23\linewidth}
        \centering
        \subcaption{SG~\cite{WanYWWLW22}}
    \end{subfigure}
        \begin{subfigure}{0.23\linewidth}
        \centering
        \subcaption{DMTN~\cite{LiuWFLQT23}}
    \end{subfigure}
    
    \includegraphics[width=.24\linewidth]{fig/4/srd/6651/IMG_6651-des3.jpg}
    \includegraphics[width=.24\linewidth]{fig/4/srd/6651/IMG_6651-homo.jpg}
    \includegraphics[width=.24\linewidth]{fig/4/srd/6651/IMG_6651-ours.jpg}
    \includegraphics[width=.24\linewidth]{fig/4/srd/6651/IMG_6651-gt.jpg}

    \begin{subfigure}{0.23\linewidth}
        \centering
        \subcaption{DeS3~\cite{Jin0YYT24}}
    \end{subfigure}
    \begin{subfigure}{0.23\linewidth}
        \centering
        \subcaption{HF~\cite{0002FZL00Z24}}
    \end{subfigure}
    \begin{subfigure}{0.23\linewidth}
        \centering
        \subcaption{Ours}
    \end{subfigure}
    \begin{subfigure}{0.23\linewidth}
        \centering
        \subcaption{GT}
    \end{subfigure}
    % \vspace{15pt}
    \caption{Visual comparisons on the SRD dataset. } 
    \label{fig:suppl.srd2}
        % \vspace{20pt}
\end{figure*}

\begin{figure*}[t]
    \centering
    
    \includegraphics[width=.19\linewidth]{fig/suppl/UIUC/DSC_0394/DSC_0394-input.jpg}
    \includegraphics[width=.19\linewidth]{fig/suppl/UIUC/DSC_0394/DSC_0394-SG.jpg}
    \includegraphics[width=.19\linewidth]{fig/suppl/UIUC/DSC_0394/DSC_0394-SF.jpg}
    \includegraphics[width=.19\linewidth]{fig/suppl/UIUC/DSC_0394/DSC_0394-homo.jpg}
    \includegraphics[width=.19\linewidth]{fig/suppl/UIUC/DSC_0394/DSC_0394-ours.jpg}

    \includegraphics[width=.19\linewidth]{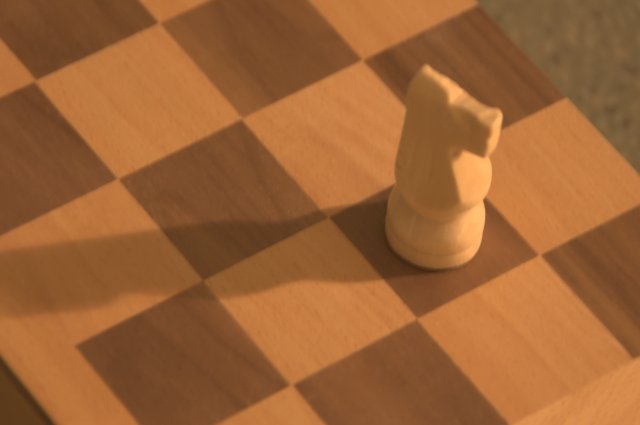}
    \includegraphics[width=.19\linewidth]{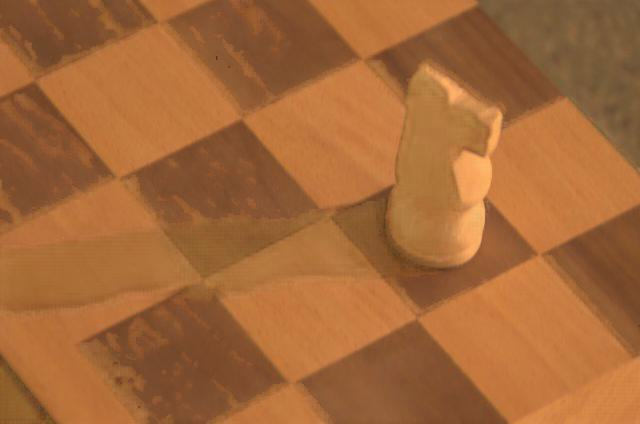}
    \includegraphics[width=.19\linewidth]{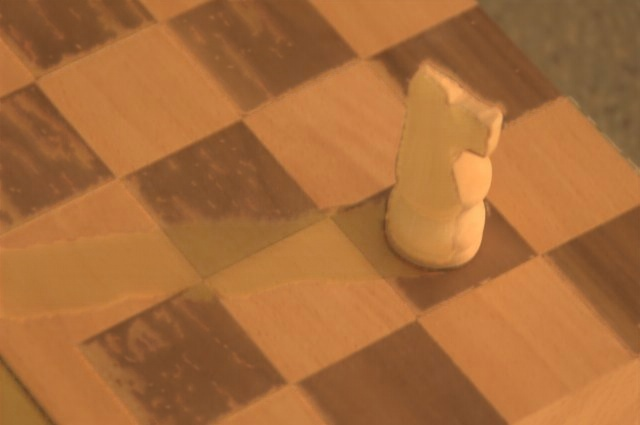}
    \includegraphics[width=.19\linewidth]{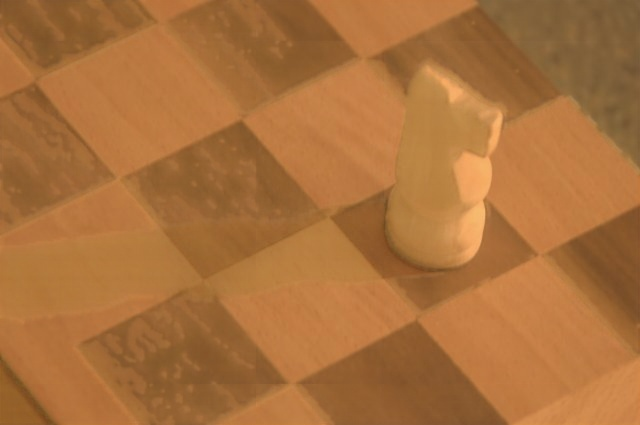}
    \includegraphics[width=.19\linewidth]{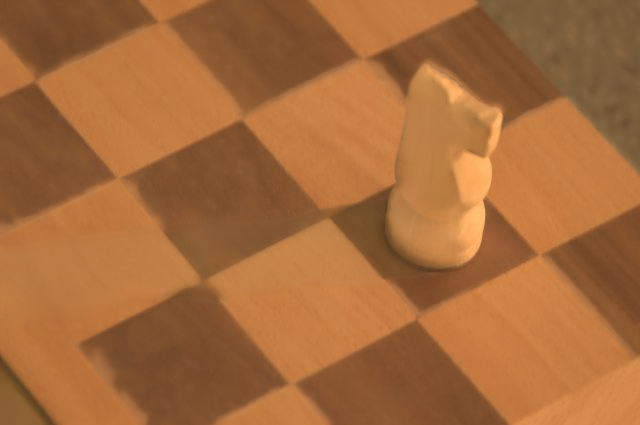}

    \includegraphics[width=.19\linewidth]{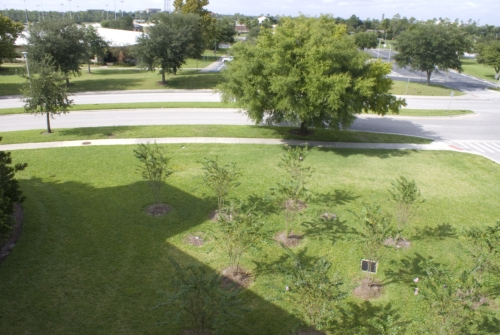}
    \includegraphics[width=.19\linewidth]{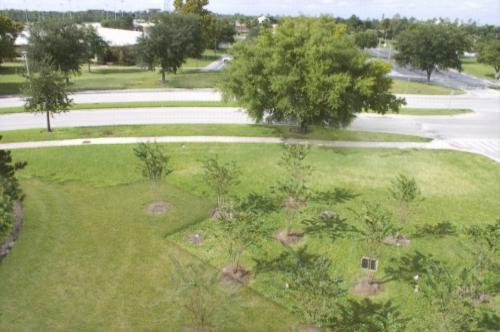}
    \includegraphics[width=.19\linewidth]{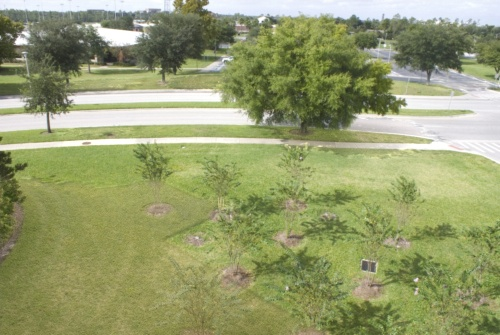}
    \includegraphics[width=.19\linewidth]{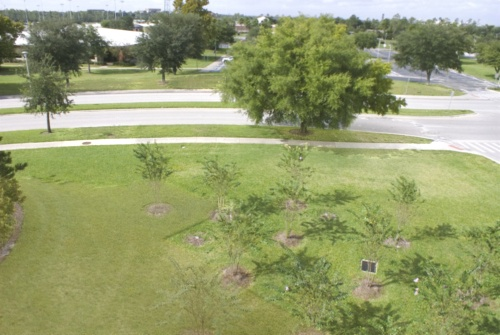}
    \includegraphics[width=.19\linewidth]{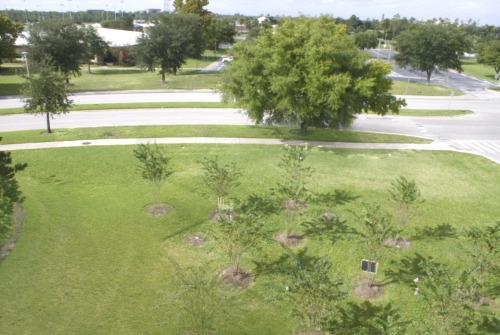}

    \includegraphics[width=.19\linewidth]{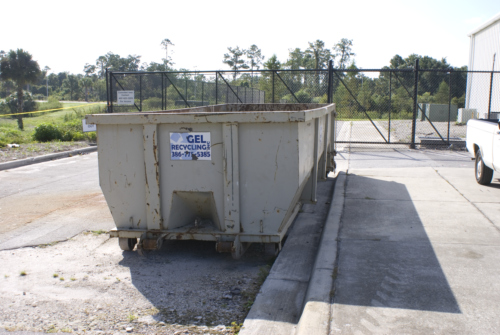}
    \includegraphics[width=.19\linewidth]{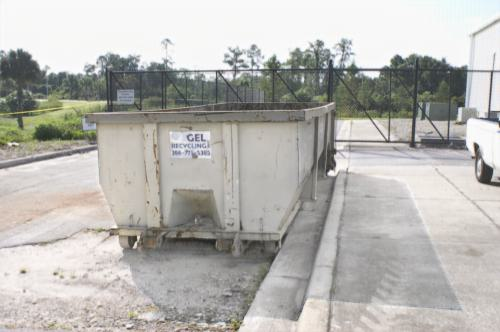}
    \includegraphics[width=.19\linewidth]{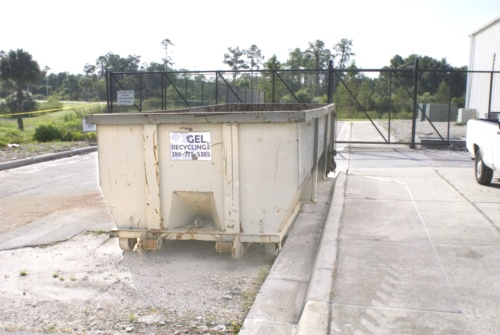}
    \includegraphics[width=.19\linewidth]{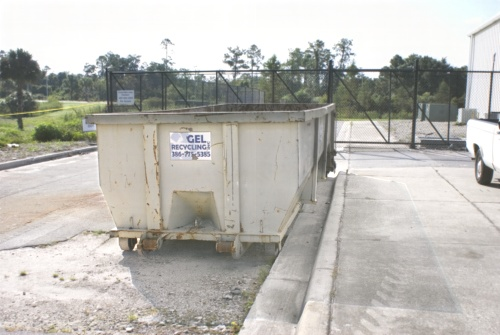}
    \includegraphics[width=.19\linewidth]{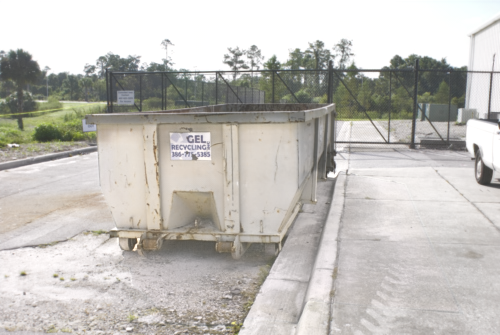}

    \includegraphics[width=.19\linewidth]{fig/suppl/UIUC/1534/DSC01534_gt.jpg}
    \includegraphics[width=.19\linewidth]{fig/suppl/UIUC/1534/DSC01534-SG.jpg}
    \includegraphics[width=.19\linewidth]{fig/suppl/UIUC/1534/DSC01534-SF.jpg}
    \includegraphics[width=.19\linewidth]{fig/suppl/UIUC/1534/DSC01534-homo.jpg}
    \includegraphics[width=.19\linewidth]{fig/suppl/UIUC/1534/DSC01534.jpg}

    \includegraphics[width=.19\linewidth, height=.15\linewidth]{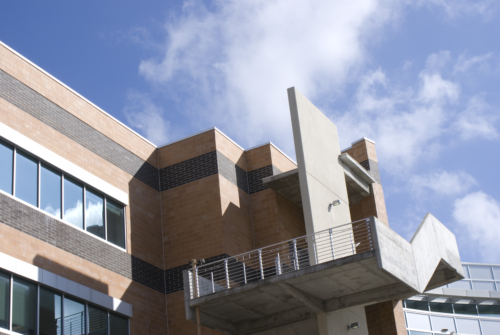}
    \includegraphics[width=.19\linewidth, height=.15\linewidth]{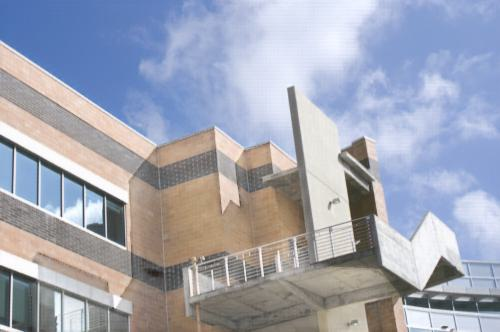}
    \includegraphics[width=.19\linewidth, height=.15\linewidth]{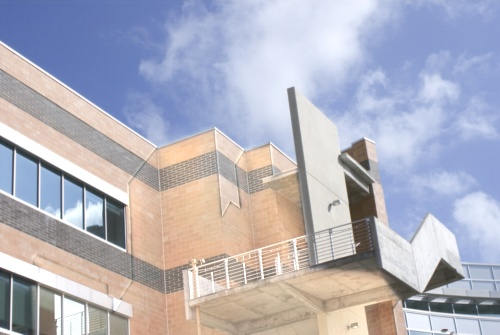}
    \includegraphics[width=.19\linewidth, height=.15\linewidth]{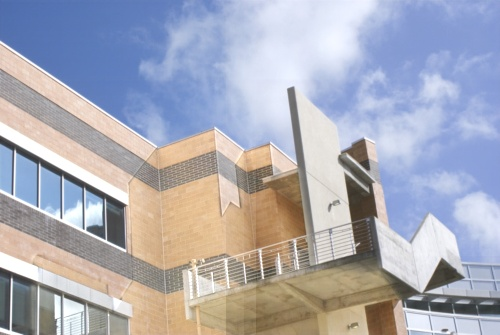}
    \includegraphics[width=.19\linewidth, height=.15\linewidth]{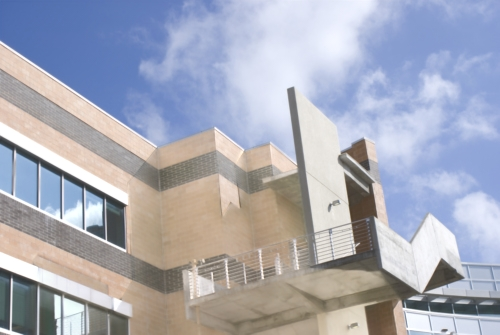}
    
    \includegraphics[width=.19\linewidth]{fig/suppl/UIUC/41835134_1793_3073_2049_3329/41835134_1793_3073_2049_3329_gt.jpg}
    \includegraphics[width=.19\linewidth]{fig/suppl/UIUC/41835134_1793_3073_2049_3329/41835134_1793_3073_2049_3329-SG.jpg}
    \includegraphics[width=.19\linewidth]{fig/suppl/UIUC/41835134_1793_3073_2049_3329/41835134_1793_3073_2049_3329-SF.jpg}
    \includegraphics[width=.19\linewidth]{fig/suppl/UIUC/41835134_1793_3073_2049_3329/41835134_1793_3073_2049_3329-homo.jpg}
    \includegraphics[width=.19\linewidth]{fig/suppl/UIUC/41835134_1793_3073_2049_3329/41835134_1793_3073_2049_3329-ours.jpg}

    \includegraphics[width=.19\linewidth]{fig/suppl/UIUC/41835134_1025_1025_1281_1281/41835134_1025_1025_1281_1281-gt.jpg}
    \includegraphics[width=.19\linewidth]{fig/suppl/UIUC/41835134_1025_1025_1281_1281/41835134_1025_1025_1281_1281-SG.jpg}
    \includegraphics[width=.19\linewidth]{fig/suppl/UIUC/41835134_1025_1025_1281_1281/41835134_1025_1025_1281_1281-SF.jpg}
    \includegraphics[width=.19\linewidth]{fig/suppl/UIUC/41835134_1025_1025_1281_1281/41835134_1025_1025_1281_1281-homo.jpg}
    \includegraphics[width=.19\linewidth]{fig/suppl/UIUC/41835134_1025_1025_1281_1281/41835134_1025_1025_1281_1281-ours.jpg}

    \begin{subfigure}{0.19\linewidth}
        \centering
        \subcaption{Input}
    \end{subfigure}
    \begin{subfigure}{0.19\linewidth}
        \centering
        \subcaption{SG~\cite{WanYWWLW22}}
    \end{subfigure}
    \begin{subfigure}{0.19\linewidth}
        \centering
        \subcaption{SF~\cite{GuoHLCW23}}
    \end{subfigure}
    \begin{subfigure}{0.19\linewidth}
        \centering
        \subcaption{HF~\cite{0002FZL00Z24}}
    \end{subfigure}
    \begin{subfigure}{0.19\linewidth}
        \centering
        \subcaption{Ours}
    \end{subfigure}

    % \vspace{15pt}
    \caption{Visual comparisons on the UIUC and UCF datasets. }
    \label{fig:suppl.ucfuiuc}
        % \vspace{20pt}
\end{figure*}
% \clearpage

\begin{figure*}[t]
    \centering
    
    \includegraphics[width=.28\linewidth]{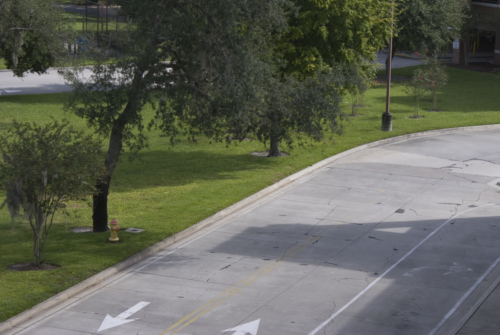}
    \includegraphics[width=.28\linewidth]{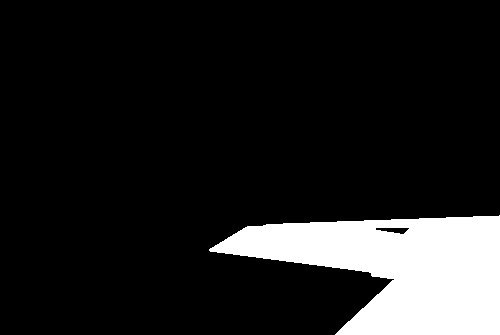}
    \includegraphics[width=.28\linewidth]{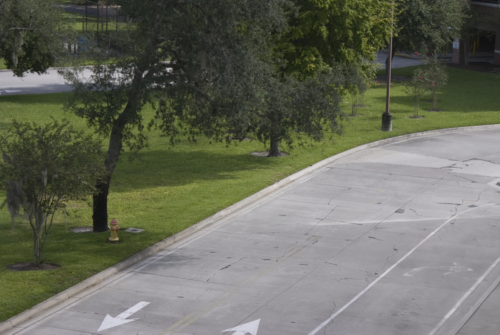}

    \begin{minipage}{.28\linewidth}
        \hfill
    \end{minipage}
    \includegraphics[width=.28\linewidth]{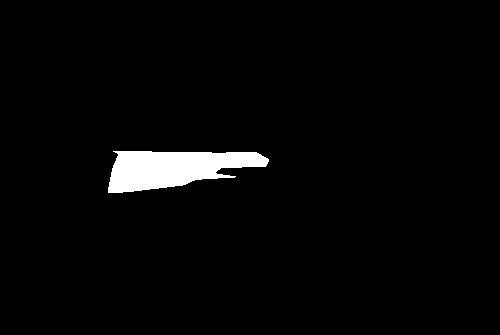}
    \includegraphics[width=.28\linewidth]{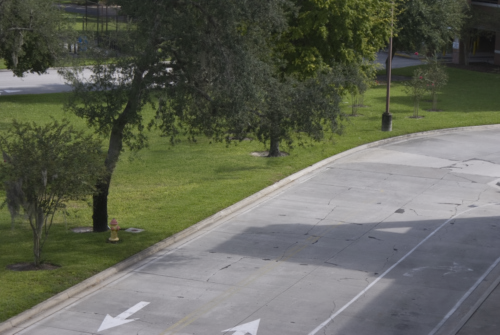}

    \includegraphics[width=.28\linewidth]{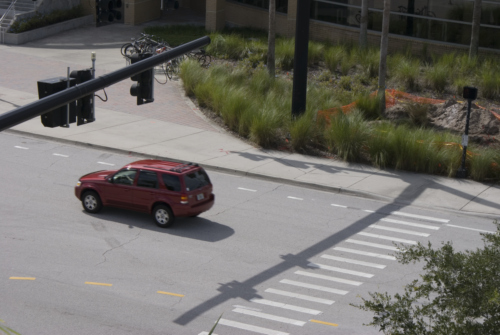}
    \includegraphics[width=.28\linewidth]{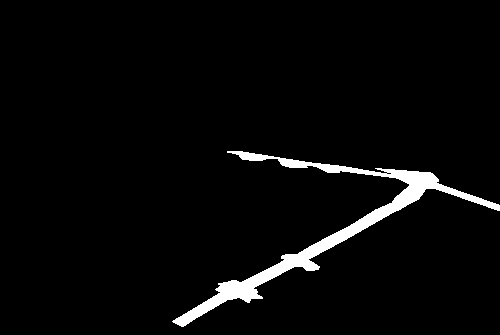}
    \includegraphics[width=.28\linewidth]{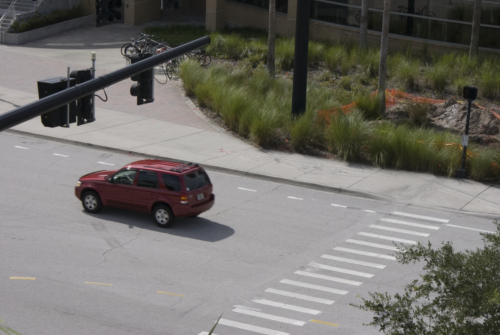}

    \begin{minipage}{.28\linewidth}
        \hfill
    \end{minipage}
    \includegraphics[width=.28\linewidth]{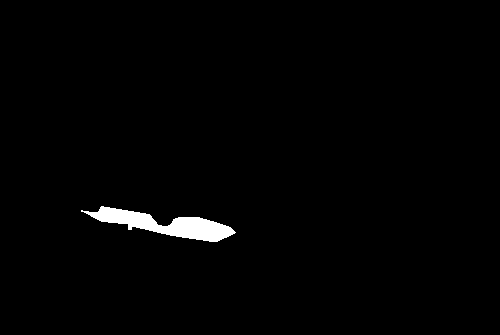}
    \includegraphics[width=.28\linewidth]{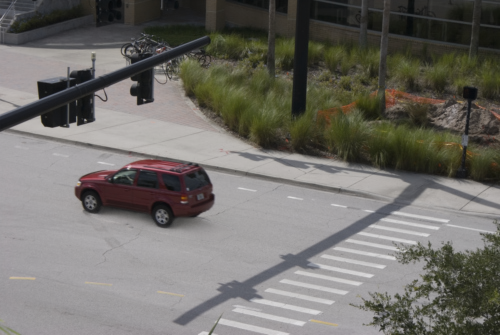}

    \includegraphics[width=.28\linewidth]{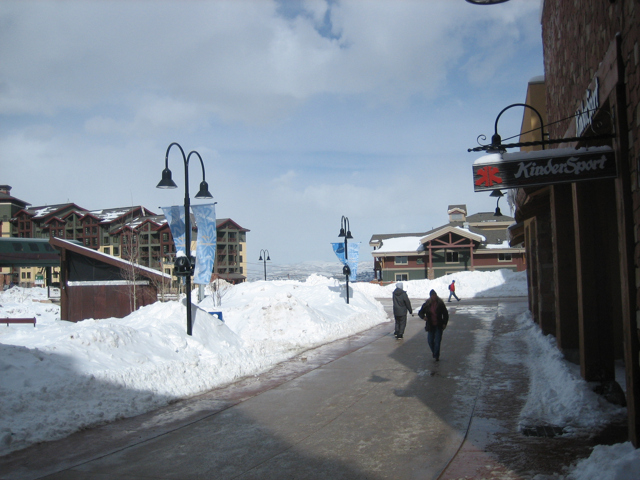}
    \includegraphics[width=.28\linewidth]{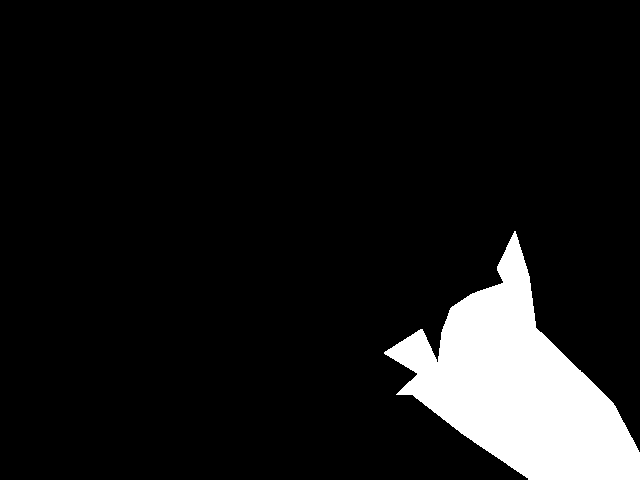}
    \includegraphics[width=.28\linewidth]{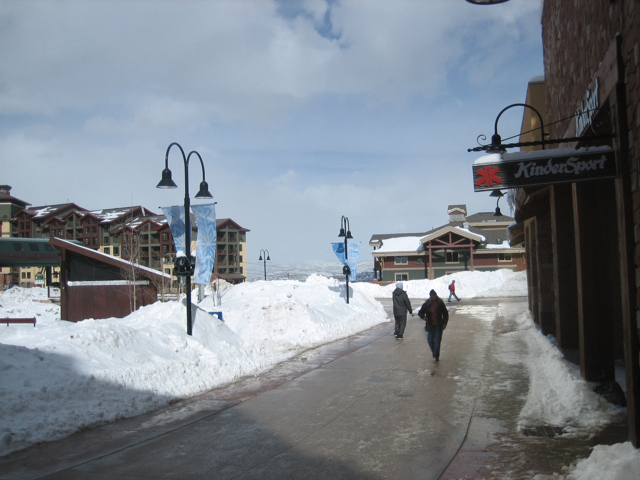}

    \begin{minipage}{.28\linewidth}
        \hfill
    \end{minipage}
    \includegraphics[width=.28\linewidth]{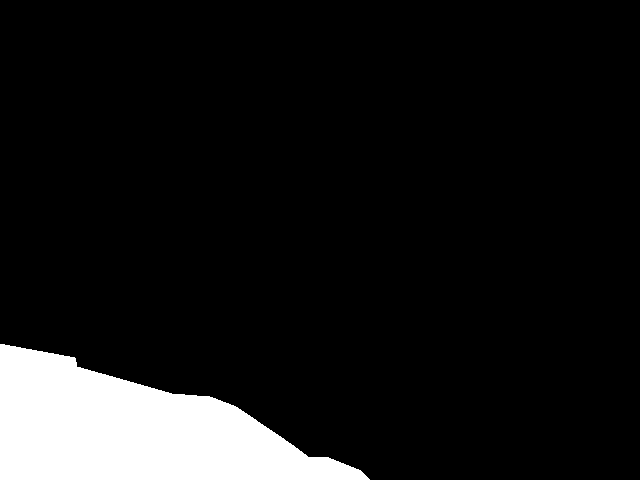}
    \includegraphics[width=.28\linewidth]{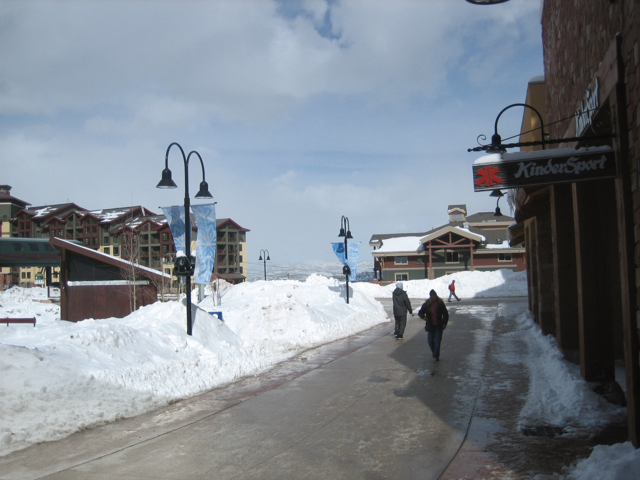}

    \begin{subfigure}{0.28\linewidth}
        \centering
        \subcaption{Input}
    \end{subfigure}
    \begin{subfigure}{0.28\linewidth}
        \centering
        \subcaption{Shadow Mask}
    \end{subfigure}
    \begin{subfigure}{0.28\linewidth}
        \centering
        \subcaption{Result}
    \end{subfigure}

    % \vspace{15pt}
    \caption{Visual results of selective shadow masks on the UCF dataset. }
    \label{fig:suppl.flexible}
        % \vspace{20pt}
\end{figure*}
